# Supplementary material for: Statistical inference for autoregressive models under heteroscedasticity of unknown form
Source: arXiv:1804.02348 ancillary file (2018-08-09)
Supplement: Supplementary file 1 [file Supplementary_material.pdf]

# SUPPLEMENTARY MATERIAL TO "STATISTICAL INFERENCE FOR AUTOREGRESSIVE MODELS UNDER HETEROSCEDASTICITY OF UNKNOWN FORM"

By Ke Zhu

*University of Hong Kong*

In this supplementary material, we give two additional examples, some additional simulation results, the applications, Lemmas B.1-B.6, and the remaining proofs for the paper.

**1. Additional examples.** In this section, we give two additional examples, which are useful but not reported in Section 5. Under the same set-up as Example 1, Examples 2 and 3 consider the cases that $g(\cdot)$ has the gradual and periodical change in the variance, respectively.

Example 2. (*A gradual change in the variance*) Let $m$ be a positive integer and $g(\cdot)$ be the continuous function

$$g(x) = e_0 + (e_1 - e_0)x^m, \tag{S.1}$$

where $x \in [0, 1]$, $e_0 > 0$, and $e_1 > 0$. Under (S.1), the variance of $\varepsilon_t$ changes gradually from $e_0^2$ to $e_1^2$ according to an $m$-th order power function. Let $\delta = e_1/e_0$. Then, some algebra shows that

$$b_1 = \frac{1}{4f^2(0)} \frac{1 + \frac{2(\delta-1)}{m+1} + \frac{(\delta-1)^2}{2m+1}}{\left(1 + \frac{\delta-1}{m+1}\right)^2}$$

$$\text{and} \quad b_3 = \frac{1 + \frac{4(\delta-1)}{m+1} + \frac{6(\delta-1)^2}{2m+1} + \frac{4(\delta-1)^3}{3m+1} + \frac{(\delta-1)^4}{4m+1}}{\left(1 + \frac{2(\delta-1)}{m+1} + \frac{(\delta-1)^2}{2m+1}\right)^2}.$$

Fig S1(a)-(f) below plot the values of all $b_i$ in terms of $\delta$ for $m = 1, 2$, and 6, respectively. From this figure, our findings are similar to those in Example 1, besides that compared with $\widehat{\theta}_{an}$ (or $\check{\theta}_{an}$), much more inefficiency in $\widehat{\theta}_n$ (or $\check{\theta}_n$) is sustained when $m > 1$ and $\delta > 1$.

Example 3. (*A periodic change in the variance*) Let $k > 1$ be a real number and $g(\cdot)$ be the periodic function

$$g(x) = \sin(\delta x) + k, \tag{S.2}$$

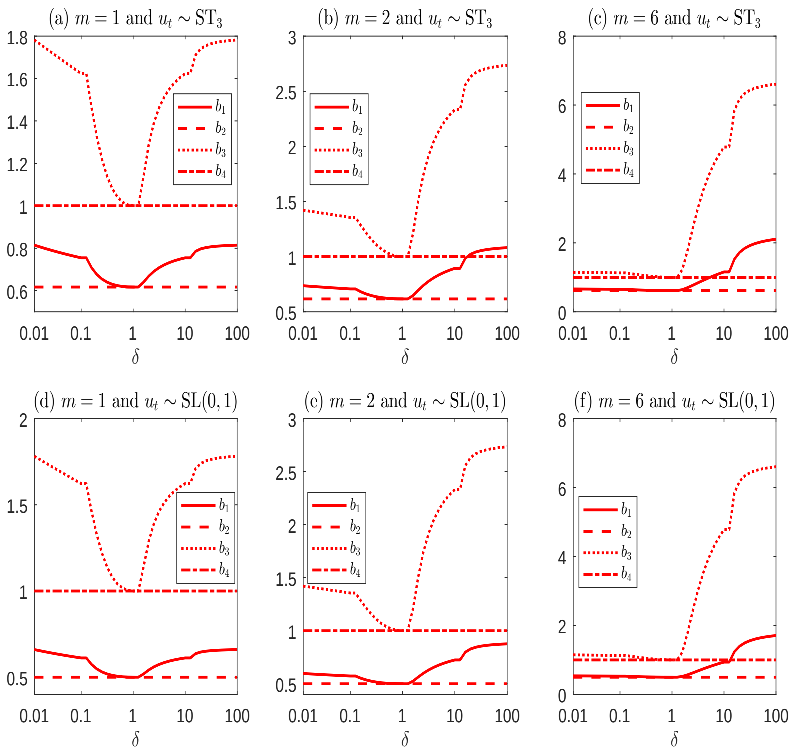


FIG S1. *The values of* $b_1$ *(solid line),* $b_2$ *(dashed line),* $b_3$ *(dash-dot line), and* $b_4$ *(dotted line) across* $\delta$

where $x \in [0,1]$ and $\delta \in [0, 4\pi]$. Under (S.2), the variance of $\varepsilon_t$ changes periodically around the equilibrium state $k^2$ with the period equal to $2\pi/\delta$. Then, some algebra shows that

$$b_1 = \frac{1}{4f^2(0)} \frac{[2k - (1/4)\sin(2\delta) - 2k\cos(\delta)]\delta + (1/2 + k^2)\delta^2}{[1 + k\delta - \cos(\delta)]^2}$$

$$\text{and } b_3 = \frac{\Delta(k,\delta)}{[2k + (1/2 + k^2)\delta - (1/4)\sin(2\delta) - 2k\cos(\delta)]^2},$$

where

$$\Delta(k,\delta) = (3/8 + 3k^2 + k^4)\delta^2 + [(4k^3 + 8k/3) - (3k^2/2 + 1/4)\sin(2\delta) + (1/32)\sin(4\delta) - (3k + 4k^3)\cos(\delta) + (k/3)\cos(3\delta)]\delta.$$

Fig S2(a)-(f) below plot the values of all $b_i$ in terms of $\delta$ for $k = 2$, 3, and 4, respectively. From this figure, our findings are similar to those in Example 1.

Moreover, we find that as the value of $k$ increases, the efficiency advantage of $\widehat{\theta}_{an}$ (or $\breve{\theta}_{an}$) over $\widehat{\theta}_n$ (or $\breve{\theta}_n$) dies away. This can be explained by the fact that the change of variance caused by the sines function is negligible when $k$ is large.

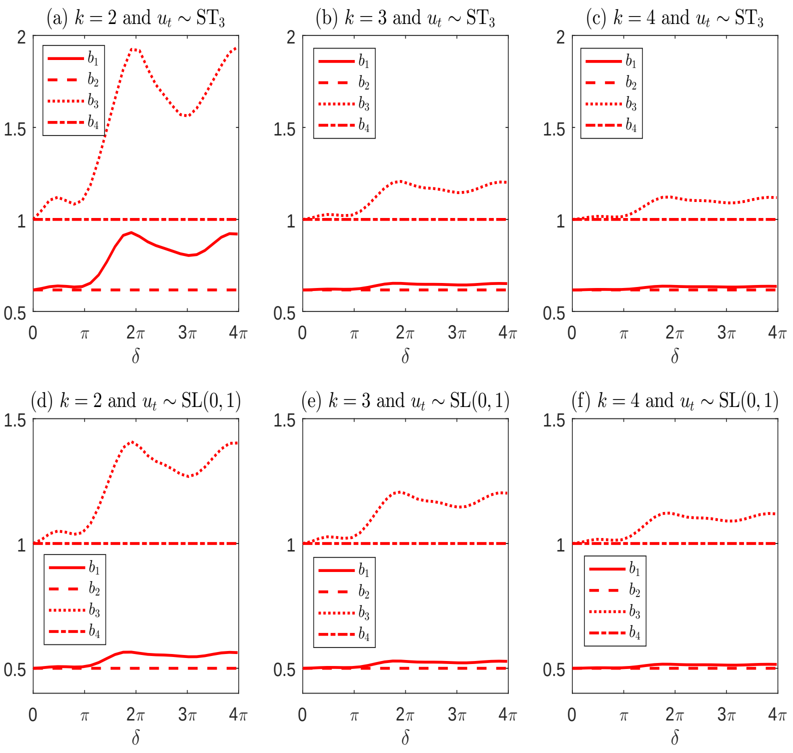


Fig S2. *The values of* $b_1$ *(solid line),* $b_2$ *(dashed line),* $b_3$ *(dash-dot line), and* $b_4$ *(dotted line) across* $\delta$

**2. Additional simulation results.** In this section, we give some additional simulation results (based on 1000 replications), which are not reported in Section 7.

First, we report the values of SE and AE of $\widehat{\theta}_n$ and $\widetilde{\theta}_{an}$ for model (7.1) with $g_t \sim$ models (7.4) and (7.5) in Tables S1 and S2, respectively. From these two tables, we have the similar findings as those in Table 1.

Second, we report the values of the sample median (SM) and sample

median of absolute deviation (SMD) of $\widehat{\theta}_n$ and $\widetilde{\theta}_{an}$ in Table S3, where

$$\text{SM} = \text{median}\{\theta_{est}^{(i)}\}_{i=1}^{1000} \quad \text{and} \quad \text{SMD} = \text{median}\{|\theta_{est}^{(i)} - \theta_0|\}_{i=1}^{1000}.$$

Here, $\theta_{est}^{(i)}$ stands for the value of either $\widehat{\theta}_n$ or $\widetilde{\theta}_{an}$ in $i$-th replication, and the true value $\theta_0 = 0.5$ as in model (7.1). Clearly, SM and SMD measure the variability of $\widehat{\theta}_n$ and $\widetilde{\theta}_{an}$, and the estimator with the value of SM (or SMD) being more close to 0.5 (or 0) is less variable than the other. From Table S3, we find that the SMs of $\widehat{\theta}_n$ and $\widetilde{\theta}_{an}$ imply that no estimator is consistently less variable than the other, while the SDMs of $\widetilde{\theta}_{an}$ are always more close to 0 than those of $\widehat{\theta}_n$, meaning that $\widetilde{\theta}_{an}$ is less variable than $\widehat{\theta}_n$ in all examined cases.

Table S1

*The values of SE and AE of $\widehat{\theta}_n$ and $\widetilde{\theta}_{an}$ for model (7.1) with $g_t \sim$ model (7.4)*

| | | | | | $\eta_t \sim$ SL(0, 1) | | $\eta_t \sim$ ST$_3$ | | $\eta_t \sim$ N(0, 1) | |
|---|---|---|---|---|---|---|---|---|---|---|
| $\alpha_\dagger$ | $\beta_\dagger$ | $\delta$ | $n$ | | $\widehat{\theta}_n$ | $\widetilde{\theta}_{an}$ | $\widehat{\theta}_n$ | $\widetilde{\theta}_{an}$ | $\widehat{\theta}_n$ | $\widetilde{\theta}_{an}$ |
| 0.0 | 0.0 | 0.2 | 100 | SE | 0.0740 | 0.0706 | 0.0799 | 0.0778 | 0.1147 | 0.1112 |
| | | | | AE | 0.0811 | 0.0783 | 0.0842 | 0.0820 | 0.1170 | 0.1131 |
| | | | 200 | SE | 0.0496 | 0.0471 | 0.0524 | 0.0510 | 0.0796 | 0.0766 |
| | | | | AE | 0.0537 | 0.0516 | 0.0574 | 0.0553 | 0.0835 | 0.0799 |
| | | 5 | 100 | SE | 0.0843 | 0.0759 | 0.0868 | 0.0795 | 0.1220 | 0.1118 |
| | | | | AE | 0.0887 | 0.0796 | 0.0923 | 0.0841 | 0.1306 | 0.1182 |
| | | | 200 | SE | 0.0554 | 0.0502 | 0.0576 | 0.0512 | 0.0878 | 0.0810 |
| | | | | AE | 0.0602 | 0.0535 | 0.0618 | 0.0556 | 0.0893 | 0.0804 |
| 0.1 | 0.8 | 0.2 | 100 | SE | 0.0841 | 0.0816 | 0.0916 | 0.0876 | 0.1228 | 0.1173 |
| | | | | AE | 0.0918 | 0.0870 | 0.1003 | 0.0951 | 0.1263 | 0.1205 |
| | | | 200 | SE | 0.0603 | 0.0559 | 0.0699 | 0.0652 | 0.0869 | 0.0839 |
| | | | | AE | 0.0625 | 0.0584 | 0.0702 | 0.0660 | 0.0895 | 0.0842 |
| | | 5 | 100 | SE | 0.0960 | 0.0843 | 0.1065 | 0.0939 | 0.1415 | 0.1243 |
| | | | | AE | 0.1044 | 0.0918 | 0.1095 | 0.0978 | 0.1401 | 0.1250 |
| | | | 200 | SE | 0.0662 | 0.0573 | 0.0729 | 0.0639 | 0.0939 | 0.0828 |
| | | | | AE | 0.0691 | 0.0599 | 0.0756 | 0.0664 | 0.0974 | 0.0862 |

Third, we report the values of $R_i$ $(i = 1, 2, 3, 4)$ for model (7.1) with $g_t \sim$ models (7.4) and (7.5) in Tables S4 and S5, respectively. Our findings from Tables S4 and S5 are similar as those from Table 2.

Fourth, we report the empirical power of all tests for model (7.6) with $g_t \sim$ models (7.4) and (7.5) in Tables S6 and S7, respectively, where $\eta_t \sim$ SL(0, 1) and their sizes correspond to the results for the case that $\kappa = 0$. Based on Tables S6 and S7, we can obtain the similar conclusions as those from Table 3.

Table S2
*The values of SE and AE of $\widehat{\theta}_n$ and $\widetilde{\theta}_{an}$ for model (7.1) with $g_t \sim$ model (7.5)*

| | | | | | $\eta_t \sim \mathrm{SL}(0,1)$ | | $\eta_t \sim \mathrm{ST}_3$ | | $\eta_t \sim \mathrm{N}(0,1)$ | |
|---|---|---|---|---|---|---|---|---|---|---|
| $\alpha_\dagger$ | $\beta_\dagger$ | $\delta$ | $n$ | | $\widehat{\theta}_n$ | $\widetilde{\theta}_{an}$ | $\widehat{\theta}_n$ | $\widetilde{\theta}_{an}$ | $\widehat{\theta}_n$ | $\widetilde{\theta}_{an}$ |
| 0.0 | 0.0 | $2\pi$ | 100 | SE | 0.0761 | 0.0728 | 0.0813 | 0.0770 | 0.1179 | 0.1129 |
| | | | | AE | 0.0825 | 0.0794 | 0.0847 | 0.0822 | 0.1195 | 0.1155 |
| | | | 200 | SE | 0.0508 | 0.0485 | 0.0560 | 0.0530 | 0.0783 | 0.0754 |
| | | | | AE | 0.0549 | 0.0522 | 0.0568 | 0.0547 | 0.0835 | 0.0797 |
| | | $4\pi$ | 100 | SE | 0.0787 | 0.0751 | 0.0800 | 0.0773 | 0.1159 | 0.1114 |
| | | | | AE | 0.0833 | 0.0807 | 0.0852 | 0.0834 | 0.1182 | 0.1146 |
| | | | 200 | SE | 0.0519 | 0.0488 | 0.0546 | 0.0522 | 0.0822 | 0.0769 |
| | | | | AE | 0.0548 | 0.0522 | 0.0574 | 0.0558 | 0.0835 | 0.0803 |
| 0.1 | 0.8 | $2\pi$ | 100 | SE | 0.0884 | 0.0827 | 0.0964 | 0.0934 | 0.1266 | 0.1186 |
| | | | | AE | 0.0951 | 0.0887 | 0.1004 | 0.0943 | 0.1280 | 0.1220 |
| | | | 200 | SE | 0.0598 | 0.0558 | 0.0691 | 0.0630 | 0.0882 | 0.0830 |
| | | | | AE | 0.0643 | 0.0592 | 0.0703 | 0.0650 | 0.0915 | 0.0860 |
| | | $4\pi$ | 100 | SE | 0.0884 | 0.0816 | 0.0961 | 0.0917 | 0.1213 | 0.1160 |
| | | | | AE | 0.0943 | 0.0886 | 0.0994 | 0.0948 | 0.1264 | 0.1212 |
| | | | 200 | SE | 0.0598 | 0.0547 | 0.0681 | 0.0621 | 0.0864 | 0.0822 |
| | | | | AE | 0.0629 | 0.0585 | 0.0716 | 0.0666 | 0.0915 | 0.0861 |

**3. Applications.** In this section, we study three U.S. economic data sets: the first differences of the monthly M1 monetary aggregate, the monthly Producer Price Index (PPI) for all commodities, and the monthly Consumer Price Index (CPI) for all urban consumers for communication. Fig S3 plots all three data sets. Both M1 and PPI data sets are taken from Feb-1959 to Jun-2016 with a length of 689 observations, and the CPI data set is taken from Feb-1998 to Jun-2016 with a length of 221 observations. Such series have been often investigated in the literature; see, Patilea and Raïssi (2014) and references therein. Particularly, Patilea and Raïssi (2014) suggested that all three series can be fitted by model (1.1) with the time-varying variance. However, they did not provide a valid way to do it.

Our aim is to use our entire statistical inference methodology based on the feasible ALADE to obtain the fitted model (1.1) for each series. First, we fit each series by a full AR(7) model, and the corresponding results are given in Table S8. From this table, we can see that each fitted AR(7) model is adequate in terms of the p-values of $S_{an}(2)$, $S_{an}(6)$ and $S_{an}(10)$. Meanwhile, we use $W_{an}$ to test the null hypothesis of the insignificance of all parameters, and then find a very strong evidence to reject this null hypothesis for each series. Since some estimated parameters seem to be insignificant, we further

TABLE S3
*The values of SM and SMD of $\widehat{\theta}_n$ and $\widetilde{\theta}_{an}$ for model (7.1)*

| | | | | | | $\eta_t \sim \mathrm{SL}(0,1)$ | | $\eta_t \sim \mathrm{ST}_3$ | | $\eta_t \sim \mathrm{N}(0,1)$ | |
|---|---|---|---|---|---|---|---|---|---|---|---|
| $g_t$ | $\alpha_\dagger$ | $\beta_\dagger$ | $\delta$ | $n$ | | $\widehat{\theta}_n$ | $\widetilde{\theta}_{an}$ | $\widehat{\theta}_n$ | $\widetilde{\theta}_{an}$ | $\widehat{\theta}_n$ | $\widetilde{\theta}_{an}$ |
| model (7.3) | 0.0 | 0.0 | 0.2 | 100 | SM | 0.4955 | 0.4967 | 0.4923 | 0.4945 | 0.4915 | 0.4936 |
| | | | | | SMD | 0.0508 | 0.0432 | 0.0548 | 0.0464 | 0.0746 | 0.0658 |
| | | | | 200 | SM | 0.5005 | 0.5007 | 0.4953 | 0.4957 | 0.4926 | 0.4961 |
| | | | | | SMD | 0.0343 | 0.0293 | 0.0422 | 0.0343 | 0.0563 | 0.0488 |
| | | | 5 | 100 | SM | 0.4977 | 0.4938 | 0.4975 | 0.5005 | 0.4967 | 0.5027 |
| | | | | | SMD | 0.0541 | 0.0445 | 0.0609 | 0.0494 | 0.0899 | 0.0733 |
| | | | | 200 | SM | 0.4998 | 0.4998 | 0.5004 | 0.4997 | 0.4955 | 0.4938 |
| | | | | | SMD | 0.0380 | 0.0313 | 0.0394 | 0.0351 | 0.0643 | 0.0512 |
| | 0.1 | 0.8 | 0.2 | 100 | SM | 0.4946 | 0.4973 | 0.4937 | 0.4945 | 0.4799 | 0.4855 |
| | | | | | SMD | 0.0588 | 0.0486 | 0.0638 | 0.0548 | 0.0852 | 0.0710 |
| | | | | 200 | SM | 0.5011 | 0.4987 | 0.4925 | 0.4938 | 0.4957 | 0.4969 |
| | | | | | SMD | 0.0428 | 0.0357 | 0.0478 | 0.0414 | 0.0660 | 0.0556 |
| | | | 5 | 100 | SM | 0.4972 | 0.4980 | 0.4968 | 0.4993 | 0.4905 | 0.4971 |
| | | | | | SMD | 0.0661 | 0.0526 | 0.0696 | 0.0595 | 0.1035 | 0.0796 |
| | | | | 200 | SM | 0.5014 | 0.5021 | 0.4906 | 0.4963 | 0.4931 | 0.4984 |
| | | | | | SMD | 0.0446 | 0.0366 | 0.0498 | 0.0416 | 0.0660 | 0.0542 |
| model (7.4) | 0.0 | 0.0 | 0.2 | 100 | SM | 0.4950 | 0.4975 | 0.4927 | 0.4949 | 0.5019 | 0.5056 |
| | | | | | SMD | 0.0470 | 0.0433 | 0.0522 | 0.0494 | 0.0749 | 0.0742 |
| | | | | 200 | SM | 0.5020 | 0.5006 | 0.4997 | 0.5009 | 0.4979 | 0.5007 |
| | | | | | SMD | 0.0323 | 0.0310 | 0.0325 | 0.0324 | 0.0566 | 0.0536 |
| | | | 5 | 100 | SM | 0.4941 | 0.4997 | 0.4994 | 0.4983 | 0.4983 | 0.4996 |
| | | | | | SMD | 0.0508 | 0.0441 | 0.0550 | 0.0509 | 0.0808 | 0.0759 |
| | | | | 200 | SM | 0.4958 | 0.4963 | 0.4994 | 0.5003 | 0.5024 | 0.5032 |
| | | | | | SMD | 0.0352 | 0.0317 | 0.0361 | 0.0325 | 0.0572 | 0.0502 |
| | 0.1 | 0.8 | 0.2 | 100 | SM | 0.4928 | 0.4921 | 0.4984 | 0.5019 | 0.4919 | 0.4920 |
| | | | | | SMD | 0.0521 | 0.0502 | 0.0626 | 0.0605 | 0.0829 | 0.0788 |
| | | | | 200 | SM | 0.4990 | 0.4989 | 0.4961 | 0.4987 | 0.4933 | 0.4936 |
| | | | | | SMD | 0.0344 | 0.0325 | 0.0435 | 0.0402 | 0.0578 | 0.0532 |
| | | | 5 | 100 | SM | 0.4949 | 0.4998 | 0.4927 | 0.4936 | 0.4937 | 0.4968 |
| | | | | | SMD | 0.0603 | 0.0522 | 0.0695 | 0.0581 | 0.0902 | 0.0847 |
| | | | | 200 | SM | 0.4957 | 0.4967 | 0.4940 | 0.4949 | 0.4917 | 0.4942 |
| | | | | | SMD | 0.0405 | 0.0338 | 0.0510 | 0.0440 | 0.0662 | 0.0570 |
| model (7.5) | 0.0 | 0.0 | $2\pi$ | 100 | SM | 0.4943 | 0.4949 | 0.4991 | 0.4998 | 0.4938 | 0.4965 |
| | | | | | SMD | 0.0492 | 0.0461 | 0.0518 | 0.0471 | 0.0754 | 0.0717 |
| | | | | 200 | SM | 0.4997 | 0.5001 | 0.4970 | 0.4974 | 0.4975 | 0.4977 |
| | | | | | SMD | 0.0321 | 0.0307 | 0.0372 | 0.0356 | 0.0559 | 0.0525 |
| | | | 5 | 100 | SM | 0.5006 | 0.5008 | 0.4963 | 0.4962 | 0.4987 | 0.4986 |
| | | | | | SMD | 0.0472 | 0.0464 | 0.0521 | 0.0521 | 0.0768 | 0.0741 |
| | | | | 200 | SM | 0.5008 | 0.5000 | 0.5000 | 0.4996 | 0.4997 | 0.5000 |
| | | | | | SMD | 0.0325 | 0.0313 | 0.0354 | 0.0347 | 0.0546 | 0.0481 |
| | 0.1 | 0.8 | $2\pi$ | 100 | SM | 0.4921 | 0.4918 | 0.4889 | 0.4879 | 0.4993 | 0.4993 |
| | | | | | SMD | 0.0516 | 0.0465 | 0.0657 | 0.0621 | 0.0804 | 0.0748 |
| | | | | 200 | SM | 0.4934 | 0.4958 | 0.4967 | 0.4978 | 0.4958 | 0.4953 |
| | | | | | SMD | 0.0380 | 0.0366 | 0.0454 | 0.0419 | 0.0615 | 0.0544 |
| | | | 5 | 100 | SM | 0.5001 | 0.4993 | 0.4914 | 0.4955 | 0.4904 | 0.4903 |
| | | | | | SMD | 0.0549 | 0.0501 | 0.0638 | 0.0602 | 0.0881 | 0.0783 |
| | | | | 200 | SM | 0.4944 | 0.4968 | 0.4969 | 0.4949 | 0.4985 | 0.4989 |
| | | | | | SMD | 0.0390 | 0.0353 | 0.0482 | 0.0426 | 0.0632 | 0.0601 |

Table S4

*The values of $R_i$ $(i = 1, 2, 3, 4)$ for model (7.1) with $g_t \sim$ model (7.4)*

| | | | | $\eta_t \sim \mathrm{SL}(0,1)$ | | | | $\eta_t \sim \mathrm{ST}_3$ | | | | $\eta_t \sim \mathrm{N}(0,1)$ | | | |
|---|---|---|---|---|---|---|---|---|---|---|---|---|---|---|---|
| $\alpha_\dagger$ | $\beta_\dagger$ | $\delta$ | $n$ | $R_1$ | $R_2$ | $R_3$ | $R_4$ | $R_1$ | $R_2$ | $R_3$ | $R_4$ | $R_1$ | $R_2$ | $R_3$ | $R_4$ |
| 0.0 | 0.0 | 0.2 | 100 | 1.0276 | 0.8820 | 0.8396 | 1.1545 | 1.0276 | 0.9836 | 0.9573 | 1.1389 | 0.9988 | 1.2958 | 1.2613 | 1.1084 |
| | | | 200 | 1.0070 | 0.8184 | 0.7776 | 1.1097 | 1.0241 | 0.8876 | 0.8631 | 1.1056 | 1.0234 | 1.3318 | 1.2812 | 1.1296 |
| | | 5 | 100 | 1.0229 | 0.9306 | 0.8381 | 1.3224 | 1.0207 | 1.0152 | 0.9326 | 1.2627 | 1.0036 | 1.3181 | 1.2127 | 1.2934 |
| | | | 200 | 1.0163 | 0.9126 | 0.8270 | 1.3696 | 1.0158 | 0.9592 | 0.8516 | 1.3358 | 1.0124 | 1.3806 | 1.2729 | 1.3416 |
| 0.1 | 0.8 | 0.2 | 100 | 1.0057 | 0.8503 | 0.8242 | 1.0749 | 1.0012 | 0.9148 | 0.8745 | 1.0522 | 0.9901 | 1.2922 | 1.2342 | 1.1150 |
| | | | 200 | 0.9732 | 0.7717 | 0.7171 | 1.0770 | 0.9659 | 0.8411 | 0.7843 | 1.0672 | 0.9874 | 1.2274 | 1.1859 | 1.0777 |
| | | 5 | 100 | 0.9956 | 0.9324 | 0.8187 | 1.2363 | 0.9845 | 0.9411 | 0.8309 | 1.2092 | 0.9980 | 1.3989 | 1.2308 | 1.2756 |
| | | | 200 | 0.9814 | 0.8390 | 0.7264 | 1.2329 | 0.9547 | 0.8677 | 0.7607 | 1.1668 | 0.9794 | 1.3654 | 1.2046 | 1.3438 |

Table S5

*The values of $R_i$ $(i = 1, 2, 3, 4)$ for model (7.1) with $g_t \sim$ model (7.5)*

| | | | | $\eta_t \sim \mathrm{SL}(0,1)$ | | | | $\eta_t \sim \mathrm{ST}_3$ | | | | $\eta_t \sim \mathrm{N}(0,1)$ | | | |
|---|---|---|---|---|---|---|---|---|---|---|---|---|---|---|---|
| $\alpha_\dagger$ | $\beta_\dagger$ | $\delta$ | $n$ | $R_1$ | $R_2$ | $R_3$ | $R_4$ | $R_1$ | $R_2$ | $R_3$ | $R_4$ | $R_1$ | $R_2$ | $R_3$ | $R_4$ |
| 0.0 | 0.0 | $2\pi$ | 100 | 1.0411 | 0.9025 | 0.8634 | 1.1568 | 1.0331 | 0.9796 | 0.9516 | 1.1528 | 1.0218 | 1.3274 | 1.2807 | 1.1754 |
| | | | 200 | 1.0242 | 0.8159 | 0.7795 | 1.1385 | 1.0288 | 0.9533 | 0.9049 | 1.1300 | 1.0003 | 1.3252 | 1.2457 | 1.1597 |
| | | $4\pi$ | 100 | 1.0376 | 0.8842 | 0.8444 | 1.1513 | 1.0293 | 0.9529 | 0.9210 | 1.1147 | 1.0169 | 1.3682 | 1.3159 | 1.1768 |
| | | | 200 | 1.0069 | 0.8470 | 0.7969 | 1.1714 | 1.0077 | 0.8745 | 0.8345 | 1.1065 | 1.0175 | 1.3272 | 1.2402 | 1.1820 |
| | 0.8 | $2\pi$ | 100 | 1.0015 | 0.8751 | 0.8202 | 1.0943 | 0.9978 | 0.9624 | 0.9360 | 1.0785 | 0.9911 | 1.3185 | 1.2368 | 1.1461 |
| | | | 200 | 0.9807 | 0.7943 | 0.7405 | 1.0440 | 0.9612 | 0.8636 | 0.7876 | 1.0950 | 0.9979 | 1.2850 | 1.2104 | 1.1367 |
| | | $4\pi$ | 100 | 0.9949 | 0.8451 | 0.7797 | 1.0558 | 0.9996 | 0.9452 | 0.9026 | 1.0733 | 1.0076 | 1.2901 | 1.2325 | 1.1396 |
| | | | 200 | 0.9891 | 0.8272 | 0.7578 | 1.0826 | 0.9596 | 0.8676 | 0.7930 | 1.0936 | 0.9939 | 1.3084 | 1.2454 | 1.1555 |

Table S6

*The power ($\times 100$) of all tests for model (7.6) with $g_t \sim$ model (7.4) and $\eta_t \sim$ SL(0, 1)*

| | | | | $\kappa = 0$ | | | | $\kappa = 0.2$ | | | | $\kappa = 0.4$ | | | |
|---|---|---|---|---|---|---|---|---|---|---|---|---|---|---|---|
| $\alpha_\dagger$ | $\beta_\dagger$ | $\delta$ | $n$ | $W_{wn}$ | $W_{an}$ | $S_w(6)$ | $S_a(6)$ | $W_{wn}$ | $W_{an}$ | $S_w(6)$ | $S_a(6)$ | $W_{wn}$ | $W_{an}$ | $S_w(6)$ | $S_a(6)$ |
| 0.0 | 0.0 | 0.2 | 100 | 4.0 | 3.7 | 2.1 | 2.0 | 55.6 | 57.6 | 7.5 | 7.4 | 97.7 | 97.9 | 46.0 | 48.8 |
| | | | 200 | 4.0 | 3.9 | 2.9 | 2.7 | 87.3 | 89.2 | 26.9 | 27.1 | 100 | 100 | 86.8 | 86.8 |
| | | 5 | 100 | 4.6 | 4.2 | 1.8 | 1.8 | 45.1 | 51.3 | 7.3 | 6.4 | 94.8 | 97.3 | 39.8 | 41.2 |
| | | | 200 | 3.5 | 3.2 | 2.7 | 3.0 | 76.3 | 84.2 | 26.4 | 26.7 | 100 | 100 | 85.2 | 84.8 |
| 0.1 | 0.8 | 0.2 | 100 | 4.5 | 3.8 | 1.2 | 2.1 | 45.6 | 49.0 | 6.4 | 6.6 | 94.3 | 96.6 | 43.0 | 46.9 |
| | | | 200 | 4.0 | 3.9 | 2.3 | 2.1 | 79.5 | 83.1 | 24.4 | 24.7 | 100 | 100 | 83.9 | 84.6 |
| | | 5 | 100 | 4.9 | 4.1 | 1.3 | 1.5 | 34.5 | 42.0 | 6.4 | 6.1 | 87.6 | 94.5 | 33.6 | 35.8 |
| | | | 200 | 4.8 | 4.1 | 2.9 | 2.4 | 69.5 | 80.4 | 21.0 | 22.1 | 99.6 | 100 | 80.7 | 81.4 |

TABLE S7

*The power (×100) of all tests for model (7.6) with $g_t \sim$ model (7.5) and $\eta_t \sim SL(0, 1)$*

| | | | | $\kappa = 0$ | | | | $\kappa = 0.2$ | | | | $\kappa = 0.4$ | | | |
|---|---|---|---|---|---|---|---|---|---|---|---|---|---|---|---|
| $\alpha_\dagger$ | $\beta_\dagger$ | $\delta$ | $n$ | $W_{wn}$ | $W_{an}$ | $S_w(6)$ | $S_a(6)$ | $W_{wn}$ | $W_{an}$ | $S_w(6)$ | $S_a(6)$ | $W_{wn}$ | $W_{an}$ | $S_w(6)$ | $S_a(6)$ |
| 0.0 | 0.0 | $2\pi$ | 100 | 3.9 | 3.0 | 1.6 | 1.8 | 53.6 | 55.8 | 7.1 | 8.2 | 96.7 | 97.2 | 43.2 | 46.0 |
| | | | 200 | 4.1 | 3.8 | 2.8 | 2.8 | 85.5 | 87.8 | 23.4 | 23.5 | 100 | 100 | 87.6 | 87.9 |
| | | $4\pi$ | 100 | 3.4 | 3.7 | 2.3 | 2.0 | 53.8 | 55.7 | 6.7 | 6.4 | 97.5 | 97.8 | 39.0 | 42.1 |
| | | | 200 | 3.6 | 3.4 | 2.9 | 2.2 | 85.5 | 88.5 | 24.3 | 22.7 | 99.8 | 100 | 86.6 | 87.5 |
| 0.1 | 0.8 | $2\pi$ | 100 | 5.2 | 5.2 | 1.0 | 1.7 | 44.0 | 46.4 | 6.2 | 6.4 | 91.9 | 94.6 | 39.9 | 43.6 |
| | | | 200 | 3.6 | 4.0 | 2.4 | 2.7 | 76.3 | 81.7 | 21.4 | 20.4 | 99.7 | 99.8 | 84.7 | 84.5 |
| | | $4\pi$ | 100 | 4.3 | 4.3 | 1.5 | 1.6 | 46.5 | 49.5 | 7.0 | 8.3 | 93.7 | 95.2 | 39.0 | 44.7 |
| | | | 200 | 3.9 | 4.0 | 2.7 | 3.1 | 76.3 | 81.9 | 19.7 | 20.2 | 99.5 | 99.8 | 84.1 | 86.0 |

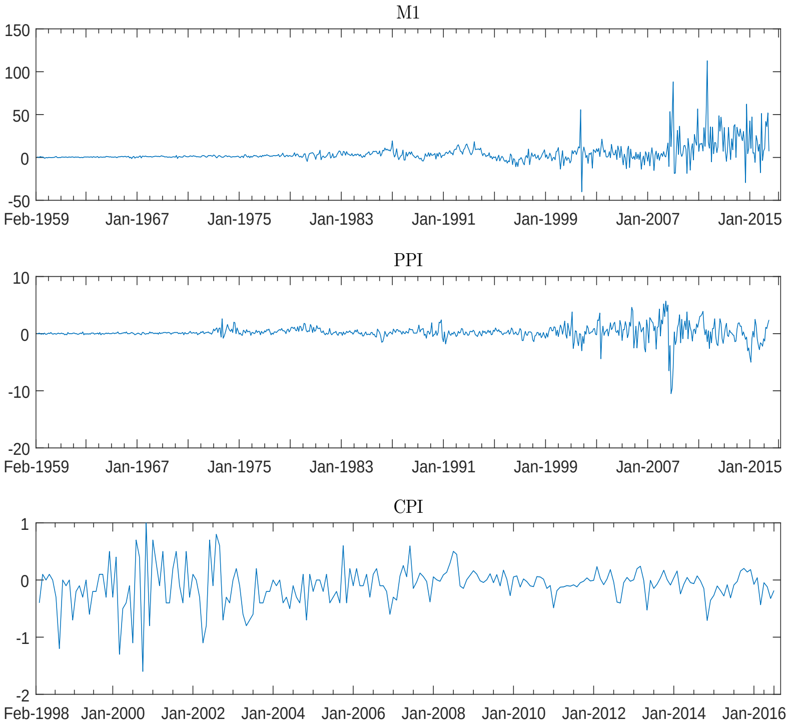


FIG S3. *The first difference of monthly M1, PPI, and CPI. Data source: The research division of the federal reserve bank of Saint Louis, http://research.stlouisfed.org/.*

use $W^*_{an}$ to detect the null hypothesis that $\phi_4 = \phi_5 = \phi_7 = 0$ for the M1 series, that $\phi_2 = \phi_4 = \phi_5 = \phi_6 = \phi_7 = 0$ for the PPI series, and that $\mu = \phi_1 = \phi_3 = \phi_4 = \phi_5 = \phi_6 = 0$ for the CPI series. The p-values of $W^*_{an}$ imply that these examined parameters are not significantly different from zeros, leading to the use of the corresponding reduced AR model to fit each series in Table S8. For each fitted reduced model, the p-values of $S_{an}(2)$, $S_{an}(6)$ and $S_{an}(10)$ indicate that it is adequate, and the p-values of $W_{an}$ show that its model parameters are all significantly different from zeros. Therefore, these reduced models are our final fitted models.

TABLE S8
*Fitted results for M1, PPI and CPI series*

| | M1 | | PPI | | CPI | |
|---|---|---|---|---|---|---|
| | Full model | Reduced model | Full model | Reduced model | Full model | Reduced model |
| $\mu$ | 0.1465 | 0.1485 | 0.0307 | 0.0409 | -0.0201 | |
| | (0.0457) | (0.0424) | (0.0138) | (0.0145) | (0.0211) | |
| $\phi_1$ | 0.3410 | 0.3352 | 0.3973 | 0.4096 | 0.1229 | |
| | (0.0516) | (0.0478) | (0.0633) | (0.0518) | (0.1044) | |
| $\phi_2$ | 0.0842 | 0.1088 | -0.0028 | | 0.1434 | 0.1400 |
| | (0.0473) | (0.0461) | (0.0516) | | (0.0744) | (0.0774) |
| $\phi_3$ | 0.2098 | 0.2120 | 0.1113 | 0.1609 | 0.0139 | |
| | (0.0482) | (0.0417) | (0.0513) | (0.0434) | (0.0585) | |
| $\phi_4$ | -0.0450 | | 0.0332 | | -0.0614 | |
| | (0.0531) | | (0.0456) | | (0.0770) | |
| $\phi_5$ | 0.0948 | | 0.0096 | | 0.0911 | |
| | (0.0558) | | (0.0514) | | (0.0683) | |
| $\phi_6$ | 0.1668 | 0.1720 | 0.0430 | | -0.0556 | |
| | (0.0414) | (0.0420) | (0.0521) | | (0.0643) | |
| $\phi_7$ | -0.0168 | | 0.0420 | | 0.1624 | 0.2040 |
| | (0.0429) | | (0.0488) | | (0.0441) | (0.0391) |
| $S_a(2)$ | 0.5249 | 0.3033 | 0.6301 | 0.2622 | 0.9222 | 0.1112 |
| $S_a(6)$ | 0.8812 | 0.6865 | 0.7086 | 0.3585 | 0.9489 | 0.2615 |
| $S_a(10)$ | 0.9520 | 0.8860 | 0.7858 | 0.5410 | 0.9147 | 0.0799 |
| $W_{an}$ | 0.0000 | 0.0000 | 0.0000 | 0.0000 | 0.0000 | 0.0000 |
| $W^*_{an}$ | 0.3396 | | 0.6616 | | 0.2336 | |

The standard deviations of the feasible ALADE are given in parentheses. The Wald test $W_{an}$ is testing for the null hypothesis of all model parameters are zeros. The Wald test $W^*_{an}$ is testing forthe null hypothesis that $\phi_4 = \phi_5 = \phi_7 = 0$ for the M1 series, that $\phi_2 = \phi_4 = \phi_5 = \phi_6 = \phi_7 = 0$ for the PPI series, and that $\mu = \phi_1 = \phi_3 = \phi_4 = \phi_5 = \phi_6 = 0$ for the CPI series. The reported values of $S_a(M)$, $W_{an}$ and $W^*_{an}$ are their p-values. In all calculations, the RW method is used with $J = 500$.

Next, we are interested in studying the structures of $g_t$ and $u_t$ based on the estimates $\widehat{g}_t$ and $\widetilde{u}_t = \widetilde{\varepsilon}_t/\widehat{g}_t$, respectively, where $\widetilde{\varepsilon}_t = y_t - Y_{t-1}'\widetilde{\theta}_{an}$. Fig S4 plots the sequence of $\{\widehat{g}_t\}$ for each series. From this figure, our findings are as follows:

(i) For the M1 series, its variance seems to be unchanged before 1979 and then rises with periodic fluctuations (roughly having the period equals to four years) between 1979 and 2002. This periodic change may be related to the change of the business cycle in U.S. After 2002, its variance keeps un-changed for about 4 years, and it starts to reach a very high level rapidly during 2007-2008, in which the financial crisis happened. After this crisis, its variance remains at this high level until recent. All these findings may imply that the business cycle in U.S. becomes vague after the financial crisis, and this could cause more challenges to make prudent monetary policies for the U.S. government.

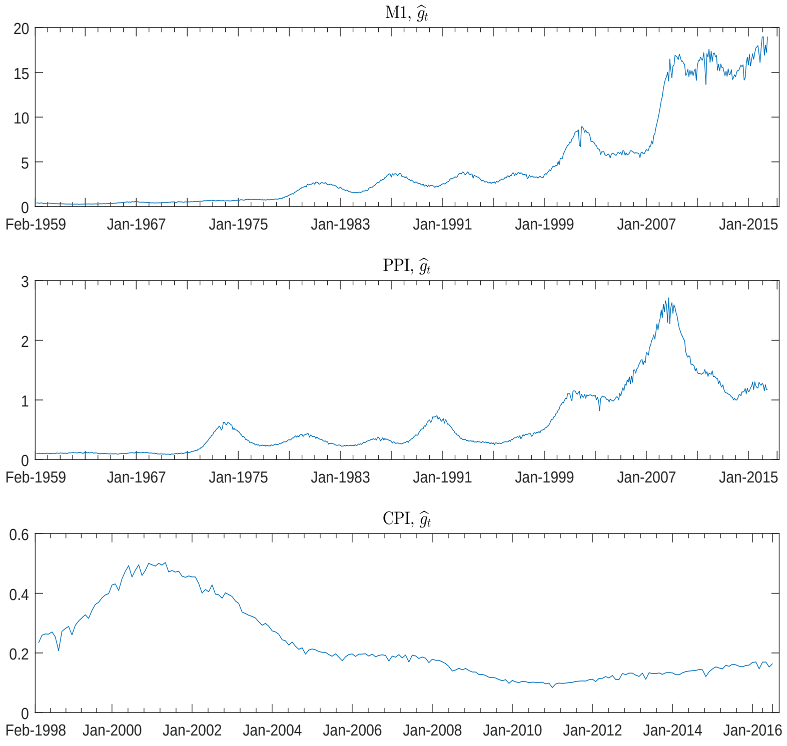


Fig S4. *The values of* $\widehat{g}_t$ *for each series*

(ii) For the PPI series, its variance structure has the similar behaviors as the M1 series before 2008. Starting from 2009, its variance declines while the variance of M1 series still stays at the high level. This finding may indicate that unlike before, the impact of monetary policies to the PPI becomes weak after the financial crisis.

(iii) For the CPI series, its variance is getting larger from 1998 to 2001, and this may be caused by the rise of M1 and PPI series during the same period. However, the influences of M1 and PPI series to CPI tend to be weaker, and the variance of CPI remains at a relatively low level after 2003. This finding may reveal that using the monetary policies to control the CPI becomes less efficient in U.S. after 2003.

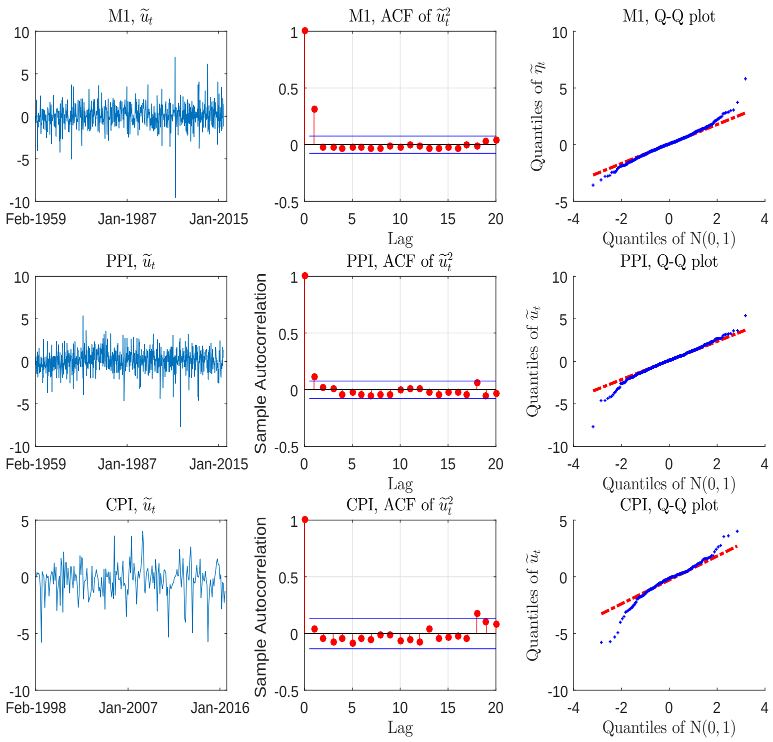


Fig S5. *Left panels: The sequences of $\widetilde{u}_t$. Middle panels: The sample ACFs of $\widetilde{u}_t^2$. Right panels: The Q-Q plot, e.g., the quantiles of $\widetilde{u}_t$ (or $\widetilde{\eta}_t$) against these of the standard normal*

Fig S5 plots the re-scaled residual $\widetilde{u}_t$ and the sample autocovariance functions (ACFs) of its square for each series. From this figure, we may deduce

that the re-scaled error $u_t$ has the ARCH effect for the M1 series, and it is i.i.d. for the PPI and CPI series. Therefore, we further use an ARCH(1) model to fit $\widetilde{u}_t$ for the M1 series, and obtain the residual $\widetilde{\eta}_t$ from this fitted ARCH(1) model. The un-reported sample ACFs of $\widetilde{\eta}_t^2$ imply that this fitted ARCH(1) model is adequate. Furthermore, Fig S5 also depicts the Q-Q plot by plotting the quantiles of $\widetilde{u}_t$ (or $\widetilde{\eta}_t$) against these of the standard normal for the PPI and CPI (or M1) series. From these Q-Q plots, we find that each $u_t$ (or $\eta_t$) has a heavier tail than the standard normal, and this demonstrates that it is reasonable to use our feasible ALADE to estimate the model for each series.

**4. Lemmas B.1-B.6.** This section give six technical lemmas in Appendix B. Lemma B.1 offers some useful technical conditions. Lemma B.2 states a general result on NED processes. Lemma B.3 is important in proving Theorem 2.1. Lemma B.4 is critical in proving Theorems 4.1-4.2 and 6.3. Lemmas B.5-B.6 are crucial in proving Theorems 6.1-6.3. The proofs of Lemmas B.1-B.6 can be found in Section 5 below.

LEMMA B.1. *Suppose Assumptions 2.1-2.2 hold and* $\sup_t \|u_t\|_{\kappa_0} < \infty$ *for some* $\kappa_0 \geq 1$. *Then,*

*(i)* $\sup_t \|y_t\|_{\kappa_0} < \infty$*;*

*(ii)* $\{y_{t-r}z_t\}$ *is* $L^{\kappa_0}$*-NED on* $\{u_t\}$ *for* $1 \leq r \leq p$*, where* $z_t \in \sigma(u_s; t - c_0 \leq s \leq t)$ *for some* $c_0 > 0$ *is uniformly bounded for all* $t$*.*

LEMMA B.2. *Suppose* $\{Z_{int}\}$ *is* $L^{2\kappa_0}$*-NED on* $\{V_t\}$ *with* $\sup_t \|Z_{int}\|_{2\kappa_0} < \infty$ *for* $i = 1, 2$ *and some* $\kappa_0 \geq 1$*. Then,* $\{Z_{1nt}Z_{2nt}\}$ *is* $L^{\kappa_0}$*-NED on* $\{V_t\}$ *with* $\sup_t \|Z_{1nt}Z_{2nt}\|_{\kappa_0} < \infty$.

LEMMA B.3. *Suppose Assumptions 2.1-2.2 hold. If* $\sup_t \|u_t\|_{2+\delta_0} < \infty$ *for some* $\delta_0 > 0$*, then*

*(i)* $\operatorname*{plim}_{n\to\infty} \frac{1}{n}\sum_{t=1}^n w_t^{-2}\left[y_{t-r} - E(y_{t-r})\right] = 0$ *for all* $1 \leq r \leq p$*;*

*(ii)* $\operatorname*{plim}_{n\to\infty} \frac{1}{n}\sum_{t=1}^n w_t^{-2}\left[y_{t-r}y_{t-s} - E(y_{t-r}y_{t-s})\right] = 0$ *for all* $1 \leq r, s \leq p$.

*If Assumption 2.4(i) and Assumption 2.5(ii) hold, then*

*(iii)* $\operatorname*{plim}_{n\to\infty} \frac{1}{n}\sum_{t=1}^n (g_t w_t)^{-1}\{f_t(0) - E[f_t(0)]\} = 0$*;*

*(iv)* $\operatorname*{plim}_{n\to\infty} \frac{1}{n}\sum_{t=1}^n (g_t w_t)^{-1}\{f_t(0)y_{t-r} - E[f_t(0)y_{t-r}]\} = 0$ *for all* $1 \leq r \leq p$*;*

*(v)* $\operatorname*{plim}_{n\to\infty} \frac{1}{n}\sum_{t=1}^n (g_t w_t)^{-1}\{f_t(0)y_{t-r}y_{t-s} - E[f_t(0)y_{t-r}y_{t-s}]\} = 0$ *for all* $1 \leq r, s \leq p$.

LEMMA B.4. *Suppose Assumption 4.1 and the conditions in Theorem 2.1 hold. Then, for any* $v_n = O_p(1)$,

(i) $\frac{1}{\sqrt{n}}\sum_{t=1}^{n} sgn\left(\varepsilon_t\left(\theta_0+\frac{v_n}{\sqrt{n}}\right)\right)=O_p(1)$;
(ii) $\frac{1}{\sqrt{n}}\sum_{t=k+1}^{n}\{P_{nt}(v_n)-E[P_{nt}(v_n)|\mathcal{F}_{t-1}]\}=o_p(1)$;
(iii) $\frac{1}{\sqrt{n}}\sum_{t=k+1}^{n}E[P_{nt}(v_n)|\mathcal{F}_{t-1}]=-2\Omega_{3k}'v_n+o_p(1)$;
(iv) $\frac{1}{\sqrt{n}}\sum_{t=k+1}^{n}Q_{nt}(v_n)=o_p(1)$,
*where*

$$P_{nt}(v)=sgn\left(u_{t-k}-\frac{v'Y_{t-k-1}}{\sqrt{n}g_{t-k}}\right)\left[sgn\left(u_t-\frac{v'Y_{t-1}}{\sqrt{n}g_t}\right)-sgn(u_t)\right],$$
$$Q_{nt}(v)=sgn(u_t)\left[sgn\left(u_{t-k}-\frac{v'Y_{t-k-1}}{\sqrt{n}g_{t-k}}\right)-sgn(u_{t-k})\right].$$

LEMMA B.5. *Suppose the conditions in Proposition A.3 hold. Then,*
(i) $(1/nb)\sum_{i=1}^{n}K_{ti}\to\int_{-\infty}^{\infty}K(x)dx=1$, *where* $t=[n\tau]$ *for any fixed* $\tau\in[0,1]$;
(ii) $\max_{1\le t,i\le n}k_{ti}=O(1/(nb))$;
(iii) $\min_{1\le t\le n}\overline{g}_t\ge\underline{C}$ *and* $\max_{1\le t\le n}\overline{g}_t\le\overline{C}$;
(iv) $\max_{1\le t\le n}E|\widetilde{g}_t-\overline{g}_t|^4=O(1/(n^2b^4))$;
(v) $\max_{1\le t\le n}E|\widetilde{g}_t-\overline{g}_t|^4=O(1/(n^2b^2))$ *if* $E(|u_t||\mathcal{F}_{t-1})=1$;
(vi) $(\min_{1\le t\le n}\widetilde{g}_t)^{-1}=O_p(1)$;
(vii) $\max_{1\le t\le n}|\widehat{g}_t-\widetilde{g}_t|=O_p(1/(\sqrt{n}b))$;
(viii) $(\min_{1\le t\le n}\widehat{g}_t)^{-1}=O_p(1)$;
(ix) $\sum_{t=1}^{n}(\widehat{g}_t-\widetilde{g}_t)^2=O_p(1/(nb^2))$;
(x) $(1/n)\sum_{t=1}^{n}|\overline{g}_t-g_t|=o(1)$.

LEMMA B.6. *Suppose the conditions in Proposition A.3 hold. Then,*
(i) $\frac{1}{\sqrt{n}}\sum_{t=1}^{n}Y_{t-1}sgn(\varepsilon_t)\left(\frac{\overline{g}_t-\widetilde{g}_t}{\overline{g}_t^2}\right)=O_p\left(\frac{1}{\sqrt{n}b^{\frac{5+\delta_4}{2}}}+\frac{1}{nb^{3+\delta_4}}+b^{\delta_4}\right)$
*for some* $\delta_4>0$; *furthermore, if* $E[|u_t||\mathcal{F}_{t-1}]=1$,
(ii) $\frac{1}{\sqrt{n}}\sum_{t=1}^{n}Y_{t-1}sgn(\varepsilon_t)\left(\frac{\overline{g}_t-\widetilde{g}_t}{\overline{g}_t^2}\right)=O_p\left(\frac{1}{nb}\right)$.

**5. Remaining proofs.** This section gives the remaining proofs for the paper.

PROOF OF PROPOSITION A.1. By noting that $\lim_{n\to\infty}\frac{1}{n}\sum_{t=1}^{n}w_t^{-2}=d_1$ and Lemma B.3, it suffices to show that
(a) $\lim_{n\to\infty}\frac{1}{n}\sum_{t=1}^{n}w_t^{-2}E(y_{t-r})=\zeta_r^{(1)}$ for all $1\le r\le p$;
(b) $\lim_{n\to\infty}\frac{1}{n}\sum_{t=1}^{n}w_t^{-2}E(y_{t-r}y_{t-s})=\zeta_{r,s}^{(1)}$ for all $1\le r,s\le p$;
(c) $\lim_{n\to\infty}\frac{1}{n}\sum_{t=1}^{n}(g_tw_t)^{-1}E[f_t(0)]=d_2$;

(d) $\lim_{n\to\infty} \frac{1}{n}\sum_{t=1}^{n}(g_t w_t)^{-1}E[f_t(0)y_{t-r}] = \zeta_r^{(2)}$ for all $1 \le r \le p$;

(e) $\lim_{n\to\infty} \frac{1}{n}\sum_{t=1}^{n}(g_t w_t)^{-1}E[f_t(0)y_{t-r}y_{t-s}] = \zeta_{r,s}^{(2)}$ for all $1 \le r, s \le p$,

where $d_1$, $d_2$, $\zeta_r^{(1)}$, $\zeta_{r,s}^{(1)}$, $\zeta_r^{(2)}$, and $\zeta_{r,s}^{(2)}$ are given in (2.2)-(2.5).

We only prove (e), since the proof of (a)-(d) is similar. By (2.1) and Assumption 2.5(iii)-(v), we have

$$\begin{aligned}
&\frac{1}{n}\sum_{t=1}^{n}\frac{E\left[f_t(0)y_{t-r}y_{t-s}\right]}{g_t w_t} \\
&= \frac{\rho^2\tau_0}{n}\sum_{t=1}^{n}\frac{1}{g_t w_t} + \rho\sum_{i=0}^{\infty}\left[\pi_i^{(1)}+\pi_i^{(2)}\right] + \sum_{i=0}^{\infty}\sum_{j=0}^{\infty}\pi_{ij}^{(3)}, \qquad \text{(S.3)}
\end{aligned}$$

where

$$\pi_i^{(1)} = \alpha_i\tau_{i+r}^{(1)}\left[\frac{1}{n}\sum_{t=1}^{n}\frac{g\left(\frac{t-r-i}{n}\right)}{g\left(\frac{t}{n}\right)w\left(\frac{t}{n}\right)}\right],\ \ \pi_i^{(2)} = \alpha_i\tau_{i+s}^{(1)}\left[\frac{1}{n}\sum_{t=1}^{n}\frac{g\left(\frac{t-s-i}{n}\right)}{g\left(\frac{t}{n}\right)w\left(\frac{t}{n}\right)}\right],$$

$$\text{and } \pi_{ij}^{(3)} = \alpha_i\alpha_j\tau_{i+r,j+s}^{(2)}\left[\frac{1}{n}\sum_{t=1}^{n}\frac{g\left(\frac{t-r-i}{n}\right)g\left(\frac{t-s-j}{n}\right)}{g\left(\frac{t}{n}\right)w\left(\frac{t}{n}\right)}\right].$$

Rewrite

$$\sum_{i=0}^{\infty}\sum_{j=0}^{\infty}\pi_{ij}^{(3)} = \sum_{i=0}^{L}\sum_{j=0}^{L}\pi_{ij}^{(3)} + \sum_{i=0}^{L}\sum_{j=L+1}^{\infty}\pi_{ij}^{(3)} + \sum_{i=L+1}^{\infty}\sum_{j=0}^{\infty}\pi_{ij}^{(3)}, \qquad \text{(S.4)}$$

where $L > 0$. By Assumptions 2.1-2.2 and 2.5(v), the first term in (S.4) satisfies that

$$\begin{aligned}
\lim_{L\to\infty}\lim_{n\to\infty}\sum_{i=0}^{L}\sum_{j=0}^{L}\pi_{ij}^{(3)} &= \lim_{L\to\infty}\lim_{n\to\infty}\left(\sum_{i=0}^{L}\sum_{j=0}^{L}\alpha_i\alpha_j\tau_{i+r,j+s}^{(2)}\right)\int_0^1\frac{g(x)}{w(x)}dx \\
&= \left(\sum_{i=0}^{\infty}\sum_{j=0}^{\infty}\alpha_i\alpha_j\tau_{i+r,j+s}^{(2)}\right)\int_0^1\frac{g(x)}{w(x)}dx, \qquad \text{(S.5)}
\end{aligned}$$

and the second term in (S.4) satisfies that uniformly in $n$,

$$\begin{aligned}
\left|\sum_{i=0}^{L}\sum_{j=L+1}^{\infty}\pi_{ij}^{(3)}\right| &\le \sum_{i=0}^{L}\sum_{j=L+1}^{\infty}\left|\alpha_i\alpha_j\tau_{i+r,j+s}^{(2)}\right| \\
&\le O(1)\left(\sum_{i=0}^{L}|\alpha_i|\right)\left(\sum_{j=L+1}^{\infty}|\alpha_j|\right) \to 0 \qquad \text{(S.6)}
\end{aligned}$$

as $L \to \infty$, due to fact that $\sum_{i=0}^{\infty} |\alpha_i| < \infty$. The similar argument as for (S.6) holds for the third term in (S.4), and then by (S.4)-(S.6) and Proposition 6.3.9 in Brockwell and Davis (1991), it follows that

$$\lim_{n\to\infty} \sum_{i=0}^{\infty}\sum_{j=0}^{\infty} \pi_{ij}^{(3)} = \left(\sum_{i=0}^{\infty}\sum_{j=0}^{\infty} \alpha_i\alpha_j\tau_{i+r,j+s}^{(2)}\right)\int_0^1 \frac{g(x)}{w(x)}dx. \tag{S.7}$$

Similarly, by Assumptions 2.1-2.2 and 2.5(iv), we can show that

$$\lim_{n\to\infty} \sum_{i=0}^{\infty} \left[\pi_i^{(1)} + \pi_i^{(2)}\right] = \left[\sum_{i=0}^{\infty} \alpha_i \left(\tau_{i+r}^{(1)} + \tau_{i+s}^{(1)}\right)\right]\int_0^1 \frac{1}{w(x)}dx, \tag{S.8}$$

and by Assumption 2.2, we have

$$\lim_{n\to\infty} \frac{1}{n}\sum_{i=0}^{\infty} \frac{1}{g_t w_t} = \int_0^1 \frac{1}{g(x)w(x)}dx. \tag{S.9}$$

Now, (e) follows directly from (S.3) and (S.7)-(S.9). This completes all of the proofs. □

Proof of Proposition A.2. Note that $\mathrm{sgn}(\varepsilon_t) = \mathrm{sgn}(u_t)$. By the Cramér-Wold device, it suffices to show that

$$\frac{1}{\sqrt{n}}\sum_{t=1}^{n} \lambda' \frac{Y_{t-1}\mathrm{sgn}(u_t)}{w_t} \to_d N(0, \lambda'\Sigma_1\lambda) \tag{S.10}$$

as $n \to \infty$, where $\lambda \in \mathcal{R}^{p+1}$ is any fixed non-zero vector. By Proposition A.1(i),

$$\begin{aligned} &\operatorname*{plim}_{n\to\infty} \frac{1}{n}\sum_{t=1}^{n} \lambda' \frac{Y_{t-1}Y_{t-1}'[\mathrm{sgn}(u_t)]^2}{w_t^2}\lambda \\ &= \operatorname*{plim}_{n\to\infty} \frac{1}{n}\sum_{t=1}^{n} \lambda' \frac{Y_{t-1}Y_{t-1}'}{w_t^2}\lambda = \lambda'\Sigma_1\lambda. \end{aligned} \tag{S.11}$$

Since $\{\lambda' Y_{t-1}\mathrm{sgn}(u_t), \mathcal{F}_t\}$ is an m.d.s. and $\|Y_{t-1}\mathrm{sgn}(u_t)\|_{2+\delta_0} < \infty$ for some $\delta_0 > 0$ by Assumption 2.4(i) and Lemma B.1(i), it follows that (S.10) holds by Corollary 5.26 in White (2001). □

Proofs of (A.5)-(A.6). To prove (A.5), we use Taylor's expansion to

re-write

$$\sum_{t=1}^{n} E(K_t|\mathcal{F}_{t-1}) = \sum_{t=1}^{n} \frac{g_t}{w_t} \int_0^{v'Y_{t-1}/(\sqrt{n}g_t)} \{F_t(s) - F_t(0)\}\, ds$$
$$= \sum_{t=1}^{n} \frac{g_t}{w_t} \int_0^{v'Y_{t-1}/(\sqrt{n}g_t)} s f_t(0) ds$$
$$+ \sum_{t=1}^{n} \frac{g_t}{w_t} \int_0^{v'Y_{t-1}/(\sqrt{n}g_t)} s[f_t(\varsigma) - f_t(0)] ds$$
$$=: \Pi_{1n} + \Pi_{2n}, \tag{S.12}$$

where $F_t(\cdot)$ is the conditional distribution of $u_t$ given $\mathcal{F}_{t-1}$, and $\varsigma$ lies between 0 and $s$.

For $\Pi_{1n}$, some algebra and Proposition A.1(ii) give us that

$$\operatorname*{plim}_{n\to\infty} \Pi_{1n} = \operatorname*{plim}_{n\to\infty} v' \left( \frac{1}{2n} \sum_{t=1}^{n} \frac{f_t(0) Y_{t-1} Y'_{t-1}}{g_t w_t} \right) v = v' \frac{\Sigma_2}{2} v \tag{S.13}$$

as $n \to \infty$.

For $\Pi_{2n}$, by Assumption 2.2 we have

$$|\Pi_{2n}| \le O(1) \sum_{t=1}^{n} \int_0^{|v'Y_{t-1}|/(\sqrt{n}\underline{C})} |s[f_t(\varsigma) - f_t(0)]|\, ds$$
$$\le O(1) \sum_{t=1}^{n} \sup_{|x| \le |v'Y_{t-1}|/(\sqrt{n}\underline{C})} |f_t(x) - f_t(0)| \int_0^{|v'Y_{t-1}|/(\sqrt{n}\underline{C})} s ds$$
$$= O\left(\frac{1}{n}\right) \sum_{t=1}^{n} |v'Y_{t-1}|^2 \sup_{|x| \le |v'Y_{t-1}|/(\sqrt{n}\underline{C})} |f_t(x) - f_t(0)|\,. \tag{S.14}$$

Choose a constant $\kappa_1 \in (0, \delta_0)$. For any $\varepsilon > 0$, there exists an $\eta_0 > 0$ such that

$$\left\| \sup_{|x| \le \eta_0} |f_t(x) - f_t(0)| \right\|_{(2+\kappa_1)/\kappa_1} < \varepsilon, \tag{S.15}$$

where (S.15) holds for all $t$ by Assumption 2.5(i) and the dominated convergence theory. Then, for any $\varepsilon, \delta > 0$,

$$P(|\Pi_{2n}| > \delta) \le P\left( |\Pi_{2n}| > \delta,\ \max_t \frac{|v'Y_{t-1}|}{\sqrt{n}\underline{C}} \le \eta_0 \right) + P\left( \max_t \frac{|v'Y_{t-1}|}{\sqrt{n}\underline{C}} > \eta_0 \right)$$

$$
\begin{aligned}
&\le P\left(|\Pi_{2n}| > \delta,\ \max_t \frac{|v'Y_{t-1}|}{\sqrt{n}\underline{C}} \le \eta_0\right) + \varepsilon \\
&\le O\left(\frac{1}{n}\right)\sum_{t=1}^{n} E\left[\|Y_{t-1}\|^2\left(\sup_{|x|\le\eta_0} |f_t(x) - f_t(0)|\right)\right] + \varepsilon \\
&\le O\left(\frac{1}{n}\right)\sum_{t=1}^{n} \|Y_{t-1}\|^2_{2+\kappa_1}\left\|\sup_{|x|\le\eta_0} |f_t(x) - f_t(0)|\right\|_{(2+\kappa_1)/\kappa_1} + \varepsilon \\
&\le O(\varepsilon)
\end{aligned}
$$

as $n \to \infty$, where the first inequality holds by the triangle's inequality, the second inequality holds since $\max_t \|Y_{t-1}\|/\sqrt{n} = o_p(1)$ by Lemma B.1(i) and a similar argument as for Pollard (1991, p.190), the third inequality holds by Markov's inequality, the fourth inequality holds by Hölder's inequality, and the fifth inequality holds by (S.15), Assumption 2.4(i), and Lemma B.1(i). Hence, it follows that $\Pi_{2n} = o_p(1)$, and together with (S.12)-(S.13), we know that (A.5) holds.

To prove (A.6), take $\kappa_2 \in (0, \min(1, \delta_0))$. Since $F_t(\cdot) \le 1$, we have

$$
\begin{aligned}
&E\left[\sum_{t=1}^{n}[K_t - E(K_t|\mathcal{F}_{t-1})]\right]^2 \\
&\le 2\sum_{t=1}^{n} EK_t^2 \\
&\le O(1)\sum_{t=1}^{n} E\left[\frac{|v'Y_{t-1}|}{\sqrt{n}}\int_0^{|v'Y_{t-1}|/\sqrt{n}} |I(\varepsilon_t \le s) - I(\varepsilon_t \le 0)| ds\right] \\
&\le O(1)\sum_{t=1}^{n} E\left[\frac{|v'Y_{t-1}|}{\sqrt{n}}\int_0^{|v'Y_{t-1}|/\sqrt{n}} [F_t(s/g_t) - F_t(0)]^{\kappa_2} ds\right] \\
&= O(1)\sum_{t=1}^{n} E\left[\frac{|v'Y_{t-1}|g_t}{\sqrt{n}}\int_0^{|v'Y_{t-1}|/(\sqrt{n}g_t)} [sf_t(\varsigma)]^{\kappa_2} ds\right] \\
&= O\left(\frac{1}{n^{1+\kappa_2/2}}\right)\sum_{t=1}^{n} E\|Y_{t-1}\|^{2+\kappa_2} \to 0 \qquad \text{(S.16)}
\end{aligned}
$$

as $n \to \infty$, where the equality in (S.16) holds by Assumption 2.2, Assumption 2.5(i), and Lemma B.1(i) with $\kappa_0 = 2 + \delta_0$. By (S.16), it follows that (A.6) holds. □

Proof of Corollary 2.1. Under (2.8), $f_t(0) = \sigma_t^{-1} f_\eta(0)$. Since $\sigma_t \ge \underline{c}$ for some $\underline{c} > 0$, Assumption 2.5(i) and (iii) hold by Assumption 2.6(i), and

Assumption 2.5(iv)-(v) hold by Assumption 2.6(i) and Assumption 2.4(ii)-(iii). Since $\{\sigma_t\}$ is $L^{2+\delta_1}$-NED on $\{u_t\}$ by Assumption 2.6(ii), it is not hard to see that $\{\sigma_t^{-1}\}$ is also $L^{2+\delta_1}$-NED on $\{u_t\}$, and hence Assumption 2.5(ii) holds. This completes the proof. □

Proof of Corollary 2.2. By Assumption 2.7 and Lemmas B.1-B.2, $\{(g_t w_t)^{-1} f_t(0) y_{t-r} y_{t-s}\}$ is $L^{1+\delta_0/2}$-NED on $\{u_t\}$ with $\sup_t \|(g_t w_t)^{-1} f_t(0) y_{t-r} y_{t-s}\|_{1+\delta_0/2} < \infty$, and hence Lemma B.3(v) holds. Similarly, we can show that Lemma B.3(iii)-(iv) hold. Hence, the proof of Theorem 2.1 above becomes valid. This completes the proof. □

Proof of Corollary 2.3. When $\phi_{i0} \equiv 0$, $Y_{t-1} = 1$. Then, we can see that Theorem 2.1 holds if Lemma B.3(iii) holds and $\lim_{n\to\infty} \frac{1}{n} \sum_{t=1}^n (g_t w_t)^{-1} E[f_t(0)] = d_2$. Clearly, this is the case under Assumption 2.8 and the law of large numbers for $L^1$-mixingales in Andrews (1988, Theorem 1). Hence, the conclusion holds. This completes the proof. □

Proof of (A.12). Since $E|w_t^*|^{2+\delta_2} < \infty$, by Hölder's and Markov's inequalities and Assumption 2.2, for all $t$ and any given $\eta > 0$, we have

$$
\begin{aligned}
&E^*\left[(w_t^* - 1)^2 I(|\lambda' J_{tn}| > \eta)\right] \\
&\quad \le \left\{E^*\left[|w_t^* - 1|^{2+\delta_2}\right]\right\}^{\frac{2}{2+\delta_2}} \left[E^* I(|\lambda' J_{tn}| > \eta)\right]^{\frac{\delta_2}{2+\delta_2}} \\
&\quad \le O(1)\left[\frac{E^*|\lambda' J_{tn}|}{\eta}\right]^{\frac{\delta_2}{2+\delta_2}} \\
&\quad \le O(1) S_n^{\frac{\delta_2}{2+\delta_2}},
\end{aligned}
$$

where $S_n = n^{-1/2} \max\limits_{1\le t\le n} \|Y_{t-1}\|$. Therefore, for any $\eta > 0$, it follows that

$$
\begin{aligned}
&\sum_{t=1}^n E^*\left[\lambda' J_{tn} J_{tn}' \lambda I(|\lambda' J_{tn}| > \eta)\right] \\
&\quad = \lambda' \left\{\frac{1}{n}\sum_{t=1}^n E^*\left[(w_t^* - 1)^2 I(|\lambda' J_{tn}| > \eta)\right] \frac{Y_{t-1} Y_{t-1}'}{w_t^2}\right\} \lambda \\
&\quad \le O(1) S_n^{\frac{\delta_2}{2+\delta_2}} \lambda' \left\{\frac{1}{n}\sum_{t=1}^n \frac{Y_{t-1} Y_{t-1}'}{w_t^2}\right\} \lambda \\
&\quad = o_p(1),
\end{aligned}
$$

where the preceding equality follows by Proposition A.1(i) and the fact that

$S_n = o_p(1)$ by Lemma B.1(i) and a similar argument as for Pollard (1991, p.190). □

PROOF OF PROPOSITION A.3. (i) By Hölder's inequality, Lemma B.1(i) and Lemma B.5(vi), (viii), and (ix), we have

$$\begin{aligned}\|z_n(\widehat{g}) - z_n(\widetilde{g})\| &\leq \left(\min_{1\leq t\leq n} \widetilde{g}_t\right)^{-1} \left(\min_{1\leq t\leq n} \widehat{g}_t\right)^{-1} \sum_{t=1}^{n} \frac{\|Y_{t-1}\|}{\sqrt{n}} |\widehat{g}_t - \widetilde{g}_t| \\ &\leq O_p(1) \left(\frac{1}{n}\sum_{t=1}^{n} \|Y_{t-1}\|^2\right)^{1/2} \left(\sum_{t=1}^{n} |\widehat{g}_t - \widetilde{g}_t|^2\right)^{1/2} \\ &= O_p\left(\frac{1}{\sqrt{nb}}\right).\end{aligned}$$

(ii) & (ii') Write

$$\begin{aligned}z_n(\widetilde{g}) - z_n(\overline{g}) &= \frac{1}{\sqrt{n}}\sum_{t=1}^{n} Y_{t-1}\mathrm{sgn}(\varepsilon_t)\left(\frac{1}{\widetilde{g}_t} - \frac{1}{\overline{g}_t}\right) \\ &= \frac{1}{\sqrt{n}}\sum_{t=1}^{n} Y_{t-1}\mathrm{sgn}(\varepsilon_t)\left(\frac{\overline{g}_t - \widetilde{g}_t}{\overline{g}_t^2}\right) \\ &\quad + \frac{1}{\sqrt{n}}\sum_{t=1}^{n} Y_{t-1}\mathrm{sgn}(\varepsilon_t)\left[\frac{(\overline{g}_t - \widetilde{g}_t)^2}{\widetilde{g}_t\overline{g}_t^2}\right]. \qquad \text{(S.17)}\end{aligned}$$

By Lemma B.1(i) and Lemma B.5(iii), (iv) and (vi), we can show that

$$\begin{aligned}&\left\|\frac{1}{\sqrt{n}}\sum_{t=1}^{n} Y_{t-1}\mathrm{sgn}(\varepsilon_t)\left[\frac{(\overline{g}_t - \widetilde{g}_t)^2}{\widetilde{g}_t\overline{g}_t^2}\right]\right\| \\ &\leq O_p(1)\sum_{t=1}^{n}\frac{\|Y_{t-1}\|}{\sqrt{n}}(\overline{g}_t - \widetilde{g}_t)^2 \\ &\leq O_p(1)\left(\sum_{t=1}^{n}\frac{\|Y_{t-1}\|^2}{n}\right)^{1/2}\left(\sum_{t=1}^{n}(\overline{g}_t - \widetilde{g}_t)^4\right)^{1/2} \\ &= O_p\left(\frac{1}{\sqrt{n}b^2}\right).\end{aligned}$$

Similarly, if $E[|u_t||\mathcal{F}_{t-1}] = 1$, by Lemma B.1(i) and Lemma B.5(iii), (v) and (vi), we have $\left\|\frac{1}{\sqrt{n}}\sum_{t=1}^{n} Y_{t-1}\mathrm{sgn}(\varepsilon_t)\left[\frac{(\overline{g}_t-\widetilde{g}_t)^2}{\widetilde{g}_t\overline{g}_t^2}\right]\right\| = O_p\left(\frac{1}{\sqrt{nb}}\right)$. Now, (ii) and (ii') follows by (S.17) and Lemma B.6.

(iii) As $\{Y_{t-1}\text{sgn}(\varepsilon_t), \mathcal{F}_t\}$ is an m.d.s., by Lemma B.1(i) and Lemma B.5(iii) and (x), it follows that

$$\begin{aligned} E\left\|z_n(\overline{g}) - z_n(g)\right\|^2 &= \frac{1}{n}\sum_{t=1}^{n} E\left\|Y_{t-1}\text{sgn}(\varepsilon_t)\left(\frac{1}{\overline{g}_t} - \frac{1}{g_t}\right)\right\|^2 \\ &\leq \left(\max_{1\leq t\leq n} E\|Y_{t-1}\|^2\right)\frac{1}{n}\sum_{t=1}^{n}\left(\frac{1}{\overline{g}_t} - \frac{1}{g_t}\right)^2 \\ &\leq O\left(\frac{1}{n}\right)\sum_{t=1}^{n}|g_t - \overline{g}_t| = o(1), \end{aligned}$$

where the last inequality has used the fact that $|g_t - \overline{g}_t| \leq g_t + \overline{g}_t \leq 2\overline{C}$. Hence, we know that (iii) holds. This completes all of proofs. □

Proof of Proposition A.4. (i) By the double expectation, Taylor's expansion, Lemma B.1(i) and Assumptions 2.2, 2.4(i), and 2.5(i), we can obtain that

$$\max_{1\leq t\leq n} E\left[\sqrt{n}|v'Y_{t-1}|I\left(|\varepsilon_t| \leq \frac{|v'Y_{t-1}|}{\sqrt{n}}\right)\right] = O(1). \tag{S.18}$$

Then, by Hölder's inequality and Lemma B.5(vi), (viii) and (vx), it follows that

$$\begin{aligned} |Z_n(\widehat{g}) - Z_n(\widetilde{g})| &\leq O_p(1)\sum_{t=1}^{n}|\widehat{g}_t - \widetilde{g}_t| \times \left|\int_0^{v'Y_{t-1}/\sqrt{n}}\{I(\varepsilon_t \leq s) - I(\varepsilon_t \leq 0)\}\, ds\right| \\ &\leq O_p(1)\sum_{t=1}^{n}|\widehat{g}_t - \widetilde{g}_t|\left[\frac{|v'Y_{t-1}|}{\sqrt{n}} I\left(|\varepsilon_t| \leq \frac{|v'Y_{t-1}|}{\sqrt{n}}\right)\right] \\ &\leq O_p(1)\left(\sum_{t=1}^{n}|\widehat{g}_t - \widetilde{g}_t|^2\right)^{1/2}\left[\sum_{t=1}^{n}\frac{|v'Y_{t-1}|^2}{n} I\left(|\varepsilon_t| \leq \frac{|v'Y_{t-1}|}{\sqrt{n}}\right)\right]^{1/2} \\ &\leq O_p\left(\frac{1}{n^{1/4}}\right)\left(\sum_{t=1}^{n}|\widehat{g}_t - \widetilde{g}_t|^2\right)^{1/2} = O_p\left(\frac{1}{n^{3/4}b}\right). \end{aligned}$$

(ii) & (ii') They can be proved by using the similar arguments as for (i).

(iii) By (S.18), Assumption 2.2, and Lemma B.5(iii) and (x), it follows that

$$E\left|Z_n(\overline{g}) - Z_n(g)\right| \leq \sum_{t=1}^{n}\left|\frac{1}{\overline{g}_t} - \frac{1}{g_t}\right| E\left|\int_0^{v'Y_{t-1}/\sqrt{n}}\{I(\varepsilon_t \leq s) - I(\varepsilon_t \leq 0)\}\, ds\right|$$

$$\leq \frac{1}{n}\sum_{t=1}^{n}\left|\frac{1}{\overline{g}_t}-\frac{1}{g_t}\right| E\left[\sqrt{n}|v'Y_{t-1}|I\left(|\varepsilon_t|\leq\frac{|v'Y_{t-1}|}{\sqrt{n}}\right)\right]$$
$$= O\left(\frac{1}{n}\right)\sum_{t=1}^{n}\left|\frac{1}{\overline{g}_t}-\frac{1}{g_t}\right| = O\left(\frac{1}{n}\right)\sum_{t=1}^{n}|\overline{g}_t-g_t| = o(1),$$

which implies that (iii) holds. This completes all of proofs. □

Proof of Corollary 5.1. First, we consider the scenario (S1). Under (S1), $\rho = 0$. By Hölder's inequality,

$$\frac{1}{4}\Sigma_2^{-1}\Sigma_1\Sigma_2^{-1} = \left(\int_0^1 \frac{g^2(x)}{w^2(x)}dx\right)\left(\int_0^1 \frac{g(x)}{w(x)}dx\right)^{-2} A \geq A,$$

where the equality holds when $w(\cdot) = g(\cdot)$ (up to a constant multiplier). Here, $A$ is the $p \times p$ matrix with $(r,s)$-th element $a_{r,s}$.

Second, we consider the scenario (S2). By some algebra,

$$n\left(\sum_{t=1}^{n}\frac{f(0)Y_{t-1}Y_{t-1}'}{g_t w_t}\right)^{-1}\left(\sum_{t=1}^{n}\frac{Y_{t-1}Y_{t-1}'}{w_t^2}\right)\left(\sum_{t=1}^{n}\frac{f(0)Y_{t-1}Y_{t-1}'}{g_t w_t}\right)^{-1}$$
$$\geq n\left(\sum_{t=1}^{n}\frac{f^2(0)Y_{t-1}Y_{t-1}'}{g_t^2}\right)^{-1}, \tag{S.19}$$

where the equality holds when $w_t = g_t$ (up to a constant multiplier). Taking $n \to \infty$, the left side of (S.19) becomes $\Sigma_2^{-1}\Sigma_1\Sigma_2^{-1}$ since $f_t(0) \equiv f(0)$, and the right side of (S.19) becomes $[f^2(0)\Sigma_{a1}]^{-1}$ by Proposition A.1(i), where $\Sigma_{a1}$ is defined in the same way as $\Sigma_1$ in (2.6) with $w_t = g_t$.

Third, we consider the scenario (S3). In this case, $\phi_{i0} \equiv 0$, and by Hölder's inequality,

$$\frac{1}{4}\Sigma_2^{-1}\Sigma_1\Sigma_2^{-1} = \frac{1}{4\tau_0^2}\left(\int_0^1 \frac{1}{w^2(x)}dx\right)\left(\int_0^1 \frac{1}{g(x)w(x)}dx\right)^{-2}$$
$$\geq \frac{1}{4\tau_0^2}\left(\int_0^1 \frac{1}{g^2(x)}dx\right)^{-1},$$

where the equality holds when $w(\cdot) = g(\cdot)$ (up to a constant multiplier). This completes all of the proofs. □

Proof of Corollary 6.1. The proof follows the similar arguments as for Theorem 2 in Xu and Phillips (2008). □

PROOF OF LEMMA B.1. Since $g(\cdot)$ is bounded by Assumption 2.2, it follows from (2.1) and Minkowski's inequality that

$$\begin{aligned}\|y_t\|_{\kappa_0} &\le |\rho| + \sum_{i=0}^{\infty} |\alpha_i| \|\varepsilon_{t-i}\|_{\kappa_0} \\ &\le O(1) + O(1) \left( \sum_{i=0}^{\infty} |\alpha_i| \right) \sup_t \|u_t\|_{\kappa_0} < \infty, \end{aligned} \tag{S.20}$$

which entails (i) holds. Next, we prove (ii) for the case that $r = p$, and the proof for other cases is similar. Take $m \ge \max(p, c_0)$. By (2.1) we can write

$$y_{t-p} = \rho + \sum_{i=0}^{m-p} \alpha_i \varepsilon_{t-p-i} + \sum_{i=m-p+1}^{\infty} \alpha_i \varepsilon_{t-p-i}.$$

Let $\mathcal{F}_{t-m}^{t+m} = \sigma(u_s; t-m \le s \le t+m\}$. By the preceding equality, we have $E\left[y_{t-p} z_t | \mathcal{F}_{t-m}^{t+m}\right] = z_t \left(\rho + \sum_{i=0}^{m-p} \alpha_i \varepsilon_{t-p-i}\right) + E\left(z_t \sum_{i=m-p+1}^{\infty} \alpha_i \varepsilon_{t-p-i} | \mathcal{F}_{t-m}^{t+m}\right)$. Hence, as for (S.20), we have

$$\begin{aligned} &\|y_{t-p} z_t - E\left[y_{t-p} z_t | \mathcal{F}_{t-m}^{t+m}\right] \|_{\kappa_0} \\ &\le O(1) \sum_{i=m-p+1}^{\infty} |\alpha_i| \cdot \|u_{t-p-i} - E(u_{t-p-i} | \mathcal{F}_{t-m}^{t+m})\|_{\kappa_0} \\ &\le O(1) \sum_{i=m-p+1}^{\infty} |\alpha_i| \cdot \|u_{t-p-i}\|_{\kappa_0} \\ &\le O(1) \left( \sum_{i=m-p+1}^{\infty} |\alpha_i| \right) \sup_t \|u_t\|_{\kappa_0} \to 0 \end{aligned}$$

as $m \to \infty$, due to the fact that $\sum_{i=1}^{\infty} |\alpha_i| < \infty$. Thus, $\{y_{t-p} z_t\}$ is $L^{\kappa_0}$-NED on $\{u_t\}$. This completes all of the proofs. □

PROOF OF LEMMA B.2. Let $\widetilde{Z}_{int} = E(Z_{int} | \mathfrak{F}_{t-m}^{t+m})$ for $i = 1, 2$. By Definition 1, $\|Z_{int} - \widetilde{Z}_{int}\|_{2\kappa_0} \le d_{int} \psi_{im}$, where $\{d_{int}\}$ are positive constants, and $\psi_{im} \to 0$ as $m \to \infty$. Then, it follows that

$$\begin{aligned} \|Z_{1nt} Z_{2nt} - \widetilde{Z}_{1nt} \widetilde{Z}_{2nt}\|_{\kappa_0} &\le \|Z_{2nt}(Z_{1nt} - \widetilde{Z}_{1nt})\|_{\kappa_0} + \|\widetilde{Z}_{1nt}(Z_{2nt} - \widetilde{Z}_{2nt})\|_{\kappa_0} \\ &\le \|Z_{2nt}\|_{2\kappa_0} \|Z_{1nt} - \widetilde{Z}_{1nt}\|_{2\kappa_0} \\ &\quad + \|\widetilde{Z}_{1nt}\|_{2\kappa_0} \|Z_{2nt} - \widetilde{Z}_{2nt}\|_{2\kappa_0} \\ &\le d_{1nt} \psi_{1m} \|Z_{2nt}\|_{2\kappa_0} + d_{2nt} \psi_{2m} \|\widetilde{Z}_{1nt}\|_{2\kappa_0} \\ &\le (d_{1nt} \|Z_{2nt}\|_{2\kappa_0} + d_{2nt} \|\widetilde{Z}_{1nt}\|_{2\kappa_0})(\psi_{1m} + \psi_{2m}), \end{aligned}$$

where the first inequality holds by the triangular inequality, the second inequality holds by Hölder's inequality, and $\|\widetilde{Z}_{1nt}\|_{2\kappa_0} \leq \|Z_{1nt}\|_{2\kappa_0} < \infty$ by Jensen's inequality. Thus, $\{Z_{1nt}Z_{2nt}\}$ is $L^{\kappa_0}$-NED by noting that

$$\begin{aligned}
&\|Z_{1nt}Z_{2nt} - E(Z_{1nt}Z_{2nt}|\mathfrak{F}_{t-m}^{t+m})\|_{\kappa_0} \\
=&\|Z_{1nt}Z_{2nt} - \widetilde{Z}_{1nt}\widetilde{Z}_{2nt} - E(Z_{1nt}Z_{2nt} - \widetilde{Z}_{1nt}\widetilde{Z}_{2nt}|\mathfrak{F}_{t-m}^{t+m})\|_{\kappa_0} \\
\leq&\|Z_{1nt}Z_{2nt} - \widetilde{Z}_{1nt}\widetilde{Z}_{2nt}\|_{\kappa_0} + \|E(Z_{1nt}Z_{2nt} - \widetilde{Z}_{1nt}\widetilde{Z}_{2nt}|\mathfrak{F}_{t-m}^{t+m})\|_{\kappa_0} \\
\leq&2\|Z_{1nt}Z_{2nt} - \widetilde{Z}_{1nt}\widetilde{Z}_{2nt}\|_{\kappa_0},
\end{aligned}$$

where the last inequality holds by Jensen's inequality. As $\sup_t \|Z_{1nt}Z_{2nt}\|_{\kappa_0} < \infty$ by Hölder's inequality, the proof is completed. □

Proof of Lemma B.3. First, we consider (ii). Under Assumptions 2.1-2.2, $\{y_{t-r}\}$ and $\{y_{t-s}w_t^{-2}\}$ are $L^{2+\delta_0}$-NED with $\sup_t \|y_{t-r}\|_{2+\delta_0} < \infty$ and $\sup_t \|y_{t-s}w_t^{-2}\|_{2+\delta_0} < \infty$ by Lemma B.1. Then, Lemma B.2 entails that $\{y_{t-r}y_{t-s}w_t^{-2}\}$ is $L^{1+\delta_0/2}$-NED with $\sup_t \|y_{t-r}y_{t-s}w_t^{-2}\|_{1+\delta_0/2} < \infty$. By the law of large numbers for $L^1$-mixingales in Andrews (1988, Theorem 1), it follows that (ii) holds. Similarly, we can show that (i) holds.

Next, we consider (v). By Assumption 2.4(i) and a similar argument as for (ii), $\{(g_tw_t)^{-1}y_{t-r}y_{t-s}\}$ is $L^{2+\delta_0/2}$-NED with $\sup_t \|(g_tw_t)^{-1}y_{t-r}y_{t-s}\|_{2+\delta_0/2} < \infty$. Moreover, by letting $\delta^* = \min(\delta_1, \delta_0/2)$, Assumption 2.5(ii), and Lemma B.2, we can show that $\{(g_tw_t)^{-1}f_t(0)y_{t-r}y_{t-s}\}$ is $L^{1+\delta^*/2}$-NED with $\sup_t \|(g_t w_t)^{-1}f_t(0)y_{t-r}y_{t-s}\|_{1+\delta^*/2} < \infty$, and hence (v) holds. Similarly, we can show that (iii)-(iv) hold. This competes all of proofs. □

Proof of Lemma B.4. (i) Denote $\Theta_v = \{v : \|v\| \leq \eta\}$ for some constant $\eta > 0$. Since $v_n = O_p(1)$, it suffices to show that

$$\sup_{v\in\Theta_v} \frac{1}{\sqrt{n}} \sum_{t=1}^{n} \left| \operatorname{sgn}\left(\varepsilon_t\left(\theta_0 + \frac{v}{\sqrt{n}}\right)\right) - \operatorname{sgn}\left(\varepsilon_t\left(\theta_0\right)\right) \right| = O_p(1), \tag{S.21}$$

due to the fact that $n^{-1/2}\sum_{t=1}^{n} \operatorname{sgn}(\varepsilon_t(\theta_0)) = O_p(1)$. By the property of the indicator function, we have

$$\begin{aligned}
&\frac{1}{\sqrt{n}} \sum_{t=1}^{n} \left| \operatorname{sgn}\left(\varepsilon_t\left(\theta_0 + \frac{v}{\sqrt{n}}\right)\right) - \operatorname{sgn}\left(\varepsilon_t\left(\theta_0\right)\right) \right| \\
&\leq \frac{2}{\sqrt{n}} \sum_{t=1}^{n} I\left(|\varepsilon_t| < \frac{|v'Y_{t-1}|}{\sqrt{n}}\right) \\
&\leq \frac{2}{\sqrt{n}} \sum_{t=1}^{n} I\left(|u_t| < \frac{\eta\|Y_{t-1}\|}{\sqrt{n}g_t}\right),
\end{aligned}$$

which entails that

$$E\left[\sup_{v\in\Theta_v}\frac{1}{\sqrt{n}}\sum_{t=1}^{n}\left|\operatorname{sgn}\left(\varepsilon_t\left(\theta_0+\frac{v}{\sqrt{n}}\right)\right)-\operatorname{sgn}\left(\varepsilon_t\left(\theta_0\right)\right)\right|\right]$$
$$\leq\frac{2}{\sqrt{n}}\sum_{t=1}^{n}EI\left(|u_t|<\frac{\eta\|Y_{t-1}\|}{\sqrt{n}g_t}\right)$$
$$\leq\frac{2}{\sqrt{n}}\sum_{t=1}^{n}E\left[\sup_x f_t(x)\frac{2\eta\|Y_{t-1}\|}{\sqrt{n}g_t}\right]<\infty, \tag{S.22}$$

where the second inequality holds by the double expectation, and the third inequality holds by Assumptions 2.2, 2.4(i), 2.5(i), and Lemma B.1. Hence, it follows that (S.21) holds.

(ii) Since $v_n = O_p(1)$, it suffices to show that

$$\sup_{v\in\Theta_v}\left|\frac{1}{\sqrt{n}}\sum_{t=k+1}^{n}\Delta_{nt}(v)\right|=o_p(1), \tag{S.23}$$

where $\Delta_{nt}(v)=P_{nt}(v)-E[P_{nt}(v)|\mathcal{F}_{t-1}]$. For each $v\in\Theta_v$, we have

$$E\left|\frac{1}{\sqrt{n}}\sum_{t=k+1}^{n}\Delta_{nt}(v)\right|^2\leq\frac{2}{n}\sum_{t=k+1}^{n}E[P_{nt}^2(v)]$$
$$\leq\frac{2}{n}\sum_{t=k+1}^{n}E\left|\operatorname{sgn}\left(u_t-\frac{v'Y_{t-1}}{\sqrt{n}g_t}\right)-\operatorname{sgn}(u_t)\right|$$
$$\leq\frac{4}{n}\sum_{t=k+1}^{n}EI\left(|u_t|<\frac{|v'Y_{t-1}|}{\sqrt{n}g_t}\right)$$
$$=O\left(\frac{1}{\sqrt{n}}\right), \tag{S.24}$$

where the first inequality holds since $\Delta_{nt}(v)$ is an m.d.s., the second and third inequalities hold by the property of the indicator function, and the last equality follows by a similar argument as for (S.22).

Moreover, for each $v_1\in\Theta_v$, let

$$U_t(v_1,\delta)=I\left(\left|u_{t-k}-\frac{v_1'Y_{t-k-1}}{\sqrt{n}g_{t-k}}\right|<\frac{\delta\|Y_{t-k-1}\|}{\sqrt{n}g_{t-k}}\right)$$
$$+I\left(\left|u_t-\frac{v_1Y_{t-1}}{\sqrt{n}g_k}\right|<\frac{\delta\|Y_{t-1}\|}{\sqrt{n}g_t}\right),$$

then for any $\delta > 0$, it is not hard to show that

$$\begin{aligned}
&\sup_{\|v-v_1\|\leq\delta}\left|\frac{1}{\sqrt{n}}\sum_{t=k+1}^{n}[\Delta_{nt}(v)-\Delta_{nt}(v_1)]\right| \\
&\leq \frac{1}{\sqrt{n}}\sum_{t=k+1}^{n}\sup_{\|v-v_1\|\leq\delta}\Big\{|P_{nt}(v)-P_{nt}(v_1)| \\
&\quad + E\left[|P_{nt}(v)-P_{nt}(v_1)|\,|\mathcal{F}_{t-1}\right]\Big\} \\
&\leq \frac{2}{\sqrt{n}}\sum_{t=k+1}^{n}\left\{U_t(v_1,\delta)+E\left[|U_t(v_1,\delta)|\,|\mathcal{F}_{t-1}\right]\right\}, \qquad \text{(S.25)}
\end{aligned}$$

By (S.25), it follows that

$$\begin{aligned}
&E\sup_{\|v-v_1\|\leq\delta}\left|\frac{1}{\sqrt{n}}\sum_{t=k+1}^{n}[\Delta_{nt}(v)-\Delta_{nt}(v_1)]\right| \leq \frac{4}{\sqrt{n}}\sum_{t=k+1}^{n}E[U_t(v_1,\delta)] \\
&\leq \frac{4\delta}{n}\sum_{t=k+1}^{n}E\left[\sup_x f_{t-k}(x)\frac{\|Y_{t-k-1}\|}{g_{t-k}}+\sup_x f_t(x)\frac{\|Y_{t-1}\|}{g_t}\right] \\
&= O(\delta). \qquad \text{(S.26)}
\end{aligned}$$

Therefore, (S.23) holds by (S.24), (S.26), and the standard arguments.

(iii) By the double expectation and Taylor's expansion, we have

$$\begin{aligned}
&\frac{1}{\sqrt{n}}\sum_{t=k+1}^{n}E\left[P_{nt}(v)\,|\mathcal{F}_{t-1}\right] \\
&= \left\{-\frac{2}{n}\sum_{t=k+1}^{n}\operatorname{sgn}\left(u_{t-k}-\frac{v'Y_{t-k-1}}{\sqrt{n}g_{t-k}}\right)f_t(\xi^*)\frac{Y'_{t-1}}{g_t}\right\}v \\
&\equiv [\Pi_{3n}+\Pi_{4n}(v)+\Pi_{5n}(v)]\,v, \qquad \text{(S.27)}
\end{aligned}$$

where $\xi^*$ lies between 0 and $v'Y_{t-1}/(\sqrt{n}g_t)$, and

$$\begin{aligned}
\Pi_{3n} &= -\frac{2}{n}\sum_{t=k+1}^{n}\operatorname{sgn}(u_{t-k})\,f_t(0)\frac{Y'_{t-1}}{g_t}, \\
\Pi_{4n}(v) &= -\frac{2}{n}\sum_{t=k+1}^{n}\left[\operatorname{sgn}\left(u_{t-k}-\frac{v'Y_{t-k-1}}{\sqrt{n}g_{t-k}}\right)-\operatorname{sgn}(u_{t-k})\right]f_t(0)\frac{Y'_{t-1}}{g_t}, \\
\Pi_{5n}(v) &= -\frac{2}{n}\sum_{t=1}^{n}\operatorname{sgn}\left(u_{t-k}-\frac{v'Y_{t-k-1}}{\sqrt{n}g_{t-k}}\right)[f_t(\xi^*)-f_t(0)]\frac{Y'_{t-1}}{g_t}.
\end{aligned}$$

For $\Pi_{3n}$, by Assumption 4.1 and the same argument as for Proposition A.1, we can show that

$$\Pi_{3n} = -2\Omega_{3k}' + o_p(1). \tag{S.28}$$

For $\Pi_{4n}(v)$, by Assumption 2.2, it is straightforward to see that

$$\sup_{v\in\Theta_v} \|\Pi_{4n}(v)\| \leq \frac{4}{n\underline{C}} \sum_{t=k+1}^{n} I\left(|u_{t-k}| \leq \frac{\eta\|Y_{t-k-1}\|}{\sqrt{n}g_{t-k}}\right) f_t(0)\|Y_{t-1}\|.$$

Then, by Holder's inequality and the double expectation, it follows that

$$\sup_{v\in\Theta_v} \|\Pi_{4n}(v)\| = o_p(1). \tag{S.29}$$

For $\Pi_{5n}(v)$, it is not hard to show that

$$\sup_{v\in\Theta_v} \|\Pi_{5n}(v)\| \leq \frac{2}{n\underline{C}} \sum_{t=k+1}^{n} \left(\sup_{|v|\leq\eta} |f_t(\xi^*) - f_t(0)|\right) \|Y_{t-1}\| = o_p(1). \tag{S.30}$$

Therefore, (iii) holds by (S.27)-(S.30) and the fact that $v_n = O_p(1)$.

(iv) Note that for each $v \in \Theta_v$, $Q_{nt}(v)$ is an m.d.s. by Assumption 2.3. Then, the proof follows by a similar argument as for (ii). This completes all of the proofs. □

Proof of Lemma B.5. We only give the proof of (iv), (vii) and (ix), since the proof of others is similar to that of Lemma A in Xu and Phillips (2008).

(iv) Under Assumptions 6.1-6.2, Theorem 4.1 in Shao and Yu (1996) gives us that

$$E\left[\widetilde{g}_t - \overline{g}_t\right]^4 \leq Cn^2 \max_{1\leq i\leq n} \|k_{ti}g_i(|u_i| - 1)\|_{4+\delta_0}^4 = O\left(\frac{1}{n^2b^4}\right)$$

for some constant $C > 0$ and all $t \geq 1$, where the last equality holds by (ii) and Assumptions 2.2 and 2.4(i).

(vii) By (ii), $|\widehat{g}_t - \widetilde{g}_t| \leq O(1/(nb))\sum_{i=1}^{n} ||\widehat{\varepsilon}_i| - |\varepsilon_i||$. Hence, it follows that

$$\begin{aligned}\max_{1\leq t\leq n} |\widehat{g}_t - \widetilde{g}_t| &\leq O\left(\frac{1}{nb}\right) \sum_{i=1}^{n} ||\widehat{\varepsilon}_i| - |\varepsilon_i|| \\ &\leq O\left(\frac{1}{nb}\right) (\widehat{\theta}_n - \theta_0) \sum_{i=1}^{n} |Y_{i-1}| = O_p\left(\frac{1}{\sqrt{n}b}\right).\end{aligned}$$

(ix) Note that $\widehat{\varepsilon}_i = \varepsilon_i - (Y_{i-1}/\sqrt{n})'\widehat{v}_n$, where $\widehat{v}_n = \sqrt{n}(\widehat{\theta}_n - \theta_0)$. By (A.3),

$$\begin{aligned}\widehat{g}_t - \widetilde{g}_t &= -\frac{\widehat{v}_n'}{\sqrt{n}} \sum_{i=1}^{n} k_{ti} Y_{i-1} \text{sgn}(\varepsilon_i) + 2\sum_{i=1}^{n} k_{ti} \int_0^{\frac{\widehat{v}_n' Y_{i-1}}{\sqrt{n}}} I(\varepsilon_i \le s) - I(\varepsilon_i \le 0) ds \\ &:= -\frac{\widehat{v}_n' s_{1nt}}{\sqrt{n}} + s_{2nt}.\end{aligned}$$

As $\widehat{v}_n = O_p(1)$ by Theorem 2.1, we only consider the case that $\|\widehat{v}_n\| \le M$ for some $M > 0$. Note that the summand of $s_{1nt}$ is an m.d.s. and by (ii),

$$\begin{aligned}|s_{2nt}| &\le \frac{2M}{\sqrt{n}} \sum_{i=1}^{n} k_{ti} \|Y_{i-1}\| I\left(|\varepsilon_i| \le \frac{M\|Y_{i-1}\|}{\sqrt{n}}\right) \\ &= O\left(\frac{1}{n^{3/2}b}\right) \sum_{i=1}^{n} \|Y_{i-1}\| I\left(|\varepsilon_i| \le \frac{M\|Y_{i-1}\|}{\sqrt{n}}\right) := O\left(\frac{1}{n^{3/2}b}\right) \sum_{i=1}^{n} W_{ni}.\end{aligned}$$

Then, it follows that

$$\begin{aligned}E\sum_{t=1}^{n} (\widehat{g}_t - \widetilde{g}_t)^2 \le\ & O\left(\frac{1}{n}\right) \sum_{t=1}^{n} \sum_{i=1}^{n} E \|k_{ti} Y_{i-1} \text{sgn}(\varepsilon_i)\|^2 \\ &+ O\left(\frac{1}{n^2 b^2}\right) E\left\{\sum_{i=1}^{n} [W_{ni} - E(W_{ni}|\mathcal{F}_{i-1})]\right\}^2 \\ &+ O\left(\frac{1}{n^2 b^2}\right) E\left\{\sum_{i=1}^{n} E(W_{ni}|\mathcal{F}_{i-1})\right\}^2 .\end{aligned} \tag{S.31}$$

Next, since $\sup_i \|Y_i\|_4 < \infty$, by Assumption 2.5, (ii) and the conditional expectation, we can show that

$$\sum_{t=1}^{n} \sum_{i=1}^{n} E \|k_{ti} Y_{i-1} \text{sgn}(\varepsilon_i)\|^2 = O\left(\frac{1}{b^2}\right), \tag{S.32}$$

$$E\left\{\sum_{i=1}^{n} [W_{ni} - E(W_{ni}|\mathcal{F}_{i-1})]\right\}^2 \le O(1) \sum_{i=1}^{n} E(W_{ni}^2) = O(\sqrt{n}), \tag{S.33}$$

$$E\left\{\sum_{i=1}^{n} E(W_{ni}|\mathcal{F}_{i-1})\right\}^2 \le O(1) E\left\{\sum_{i=1}^{n} \frac{\|Y_{i-1}\|^2}{\sqrt{n}}\right\}^2 = O(n). \tag{S.34}$$

Hence, by (S.31)-(S.34), we have $E\sum_{t=1}^{n} (\widehat{g}_t - \widetilde{g}_t)^2 = O\left(\frac{1}{nb^2}\right) + O\left(\frac{1}{n^{3/2}b^2}\right) = O\left(\frac{1}{nb^2}\right)$. Now, (ix) follows directly from Markov's inequality. This completes all of proofs. □

Proof of Lemma B.6. When $E[|u_t||\mathcal{F}_{t-1}] = 1$, $Y_{t-1}\mathrm{sgn}(\varepsilon_t)\left(\frac{\overline{g}_t - \widetilde{g}_t}{\overline{g}_t^2}\right)$ is an m.d.s., and the proof of (ii) follows the similar arguments as for Theorem 2 in Xu and Phillips (2008).

To prove (i), without loss of generality, we only show that

$$\Upsilon_n := \frac{1}{\sqrt{n}} \sum_{t=1}^{n} y_{t-1}\mathrm{sgn}(u_t)\left(\frac{\overline{g}_t - \widetilde{g}_t}{\overline{g}_t^2}\right) = o_p(1). \tag{S.35}$$

Let $\varpi_t = \frac{y_{t-1}\mathrm{sgn}(u_t)}{\overline{g}_t^2}$, $\varrho_{nt} = \sum_{i=1}^{t-1} k_{ti} g_i(|u_i|-1)$ and $\varsigma_{nt} = \sum_{i=t+1}^{n} k_{ti} g_i(|u_i|-1)$. Then, $\Upsilon_n$ can be re-written as

$$\Upsilon_n = \frac{1}{\sqrt{n}} \sum_{t=1}^{n} \varpi_t \varrho_{nt} + \frac{1}{\sqrt{n}} \sum_{t=1}^{n} \varpi_t \varsigma_{nt} := \Upsilon_{1n} + \Upsilon_{2n}.$$

For $\Upsilon_{1n}$, it is an m.d.s. by Assumption 2.3, hence we have

$$E\left[\Upsilon_{1n}^2\right] = \frac{1}{n}\sum_{t=1}^{n} E(\varpi_t \varrho_{nt})^2 \le \frac{1}{n}\sum_{t=1}^{n} \|\varpi_t\|_4^2 \|\varrho_{nt}\|_4^2,$$

where the last inequality holds by Hölder's inequality. By Assumption 2.4(i), Lemma B.1(i) and Lemma B.5(iii), we can show that $\max_{1\le t\le n}\|\varpi_t\|_4^2 < \infty$; and meanwhile, by Assumptions 2.2 and 6.1-6.2 and Theorem 4.1 in Shao and Yu (1996), we have $\|\varrho_{nt}\|_4 \le C\sqrt{t}\max_{1\le i\le n}\|k_{ti}(|u_i|-1)\|_{4+\delta_0}$ for some $C > 0$. Hence, by Lemma B.5(ii), it follows that

$$\begin{aligned} E\left[\Upsilon_{1n}^2\right] &\le O\left(\frac{1}{n}\right)\sum_{t=1}^{n}\left[\sqrt{t}\max_{1\le i\le n}\|k_{ti}(|u_i|-1)\|_{4+\delta}\right]^2 \\ &= O\left(\frac{1}{n^3 b^2}\right)\sum_{t=1}^{n} t = O\left(\frac{1}{nb^2}\right). \end{aligned} \tag{S.36}$$

For $\Upsilon_{2n}$, we have

$$\Upsilon_{2n}^2 = \frac{1}{n}\sum_{t=1}^{n}\sum_{t'=1}^{n} \varpi_t\varsigma_{nt}\varpi_{t'}\varsigma_{nt'} := \frac{1}{n}\Xi_{1n} + \frac{1}{n}\Xi_{2n} + \frac{1}{n}\Xi_{3n},$$

where $\Xi_{1n} = \sum_{t=1}^{n}\sum_{t'>t} \varpi_t\varsigma_{nt}\varpi_{t'}\varsigma_{nt'}$, $\Xi_{2n} = \sum_{t=1}^{n}\sum_{t'=t} \varpi_t\varsigma_{nt}\varpi_{t'}\varsigma_{nt'}$, and $\Xi_{3n} = \sum_{t'=1}^{n}\sum_{t>t'} \varpi_t\varsigma_{nt}\varpi_{t'}\varsigma_{nt'}$. We now consider $\frac{1}{n}\Xi_{1n}$. Choose a positive

integer $l_n$ such that $l_n^{-1} = o(1)$. Write

$$\begin{aligned}
\Xi_{1n} &= \sum_{t=1}^{n}\sum_{t'>t} \varpi_t \left(\varsigma_{1nt} + \varsigma_{2nt}\right) \varpi_{t'} \left(\varsigma_{1nt'} + \varsigma_{2nt'}\right) \\
&= \sum_{t=1}^{n}\sum_{t'>t} \varpi_t \varsigma_{1nt} \varpi_{t'} \varsigma_{1nt'} + \sum_{t=1}^{n}\sum_{t'>t} \varpi_t \varsigma_{1nt} \varpi_{t'} \varsigma_{2nt'} \\
&\quad + \sum_{t=1}^{n}\sum_{t'>t} \varpi_t \varsigma_{2nt} \varpi_{t'} \varsigma_{1nt'} + \sum_{t=1}^{n}\sum_{t'>t} \varpi_t \varsigma_{2nt} \varpi_{t'} \varsigma_{2nt'} \\
&:= \Xi_{11n} + \Xi_{12n} + \Xi_{13n} + \Xi_{14n}, \qquad \text{(S.37)}
\end{aligned}$$

where $\varsigma_{1nt} = \sum_{i=t+1}^{t'-1} k_{ti} g_i(|u_i| - 1)$, $\varsigma_{2nt} = \sum_{i=t'}^{n} k_{ti} g_i(|u_i| - 1)$, $\varsigma_{1nt'} = \sum_{i=t'+1}^{t'+l_n-1} k_{t'i} g_i(|u_i| - 1)$, and $\varsigma_{2nt'} = \sum_{i=t'+l_n}^{n} k_{t'i} g_i(|u_i| - 1)$.

First, as for (S.36), it is not hard to show that

$$\begin{aligned}
\left| E\left(\frac{1}{n}\Xi_{11n}\right)\right| &\leq \frac{1}{n}\sum_{t=1}^{n}\sum_{t'>t} \|\varpi_t\|_4 \|\varpi_{t'}\|_4 \|\varsigma_{1nt}\|_4 \|\varsigma_{1nt'}\|_4 \\
&\leq O\left(\frac{1}{n^3 b^2}\right) \sum_{t=1}^{n}\sum_{t'>t} \sqrt{(t'-t-1)l_n} = O\left(\frac{\sqrt{l_n}}{\sqrt{n} b^2}\right). \qquad \text{(S.38)}
\end{aligned}$$

Second, since $E\varsigma_{2nt'} = 0$, we have

$$\begin{aligned}
\left| E\left(\frac{1}{n}\Xi_{12n}\right)\right| &= \left| \frac{1}{n}\sum_{t=1}^{n}\sum_{t'>t} Cov(\varpi_t \varpi_{t'} \varsigma_{1nt}, \varsigma_{2nt'}) \right| \\
&\leq \frac{1}{n}\sum_{t=1}^{n}\sum_{t'>t} \|\varpi_t \varpi_{t'} \varsigma_{1nt}\|_{(4+\delta_0)/3} \|\varsigma_{2nt'}\|_{4+\delta_0} \left[\alpha_u(l_n)\right]^{\frac{\delta_0}{4+\delta_0}} \\
&\leq \frac{1}{n}\sum_{t=1}^{n}\sum_{t'>t} \|\varpi_t\|_{4+\delta_0} \|\varpi_{t'}\|_{4+\delta_0} \|\varsigma_{1nt}\|_{4+\delta_0} \|\varsigma_{2nt'}\|_{4+\delta_0} \left[\alpha_u(l_n)\right]^{\frac{\delta_0}{4+\delta_0}} \\
&\leq O\left(\frac{1}{n^3 b^2}\right) \sum_{t=1}^{n}\sum_{t'>t} \sqrt{(t'-t-1)n} \left[\alpha_u(l_n)\right]^{\frac{\delta_0}{4+\delta_0}} \\
&\leq O\left(\frac{\left[\alpha_u(l_n)\right]^{\delta_0/(4+\delta_0)}}{b^2}\right) = O\left(\frac{1}{l_n^2 b^2}\right), \qquad \text{(S.39)}
\end{aligned}$$

where the first inequality holds by Davydov's inequality in Davydov (1968), the second inequality holds by Hölder's inequality, the third inequality follows by the similar arguments as for (S.36), and the last equality holds by

Assumption 6.2. Third, write

$$\left|E\left(\frac{1}{n}\Xi_{13n}\right)\right| = \left|\frac{1}{n}\sum_{t=1}^{n}\sum_{t'>t} E\left[\varpi_t(\varsigma_{21nt}+\varsigma_{22nt})\varpi_{t'}\varsigma_{1nt'}\right]\right|$$
$$= \left|\frac{1}{n}\sum_{t=1}^{n}\sum_{t'>t}\left\{E\left[\varpi_t\varsigma_{21nt}\varpi_{t'}\varsigma_{1nt'}\right] + Cov(\varpi_t\varpi_{t'}\varsigma_{1nt'}, \varsigma_{22nt})\right\}\right|,$$

where $\varsigma_{21nt} = \sum_{i=t'}^{t'+2l_n-3} k_{ti}g_i(|u_i|-1)$ and $\varsigma_{22nt} = \sum_{i=t'+2l_n-2}^{n} k_{ti}g_i(|u_i|-1)$. By the similar arguments as for (S.38) and (S.39), we have that $\left|\frac{1}{n}\sum_{t=1}^{n}\sum_{t'>t} E\left[\varpi_t\varsigma_{21nt}\varpi_{t'}\varsigma_{1nt'}\right]\right| = O\left(\frac{l_n}{nb^2}\right)$ and $\left|\frac{1}{n}\sum_{t=1}^{n}\sum_{t'>t} Cov(\varpi_t\varpi_{t'}\varsigma_{1nt'}, \varsigma_{22nt})\right| = O\left(\frac{1}{\sqrt{n}l_n^{3/2}b^2}\right)$, respectively. Hence,

$$\left|E\left(\frac{1}{n}\Xi_{13n}\right)\right| = O\left(\frac{l_n}{nb^2}\right) + O\left(\frac{1}{\sqrt{n}l_n^{3/2}b^2}\right). \tag{S.40}$$

Fourth, write

$$\left|E\left(\frac{1}{n}\Xi_{14n}\right)\right| = \left|\frac{1}{n}\sum_{t=1}^{n}\sum_{t'>t} E\left[\varpi_t(\varsigma_{23nt}+\varsigma_{24nt})\varpi_{t'}\varsigma_{2nt'}\right]\right|$$
$$= \left|\frac{1}{n}\sum_{t=1}^{n}\sum_{t'>t}\left\{Cov\left(\varpi_t\varpi_{t'}\varsigma_{23nt}, \varsigma_{2nt'}\right) + Cov(\varpi_t\varpi_{t'}, \varsigma_{24nt}\varsigma_{2nt'})\right\}\right|,$$

where $\varsigma_{23nt} = \sum_{i=t'}^{t'+l_n/2-1} k_{ti}g_i(|u_i|-1)$ and $\varsigma_{24nt} = \sum_{i=t'+l_n/2}^{n} k_{ti}g_i(|u_i|-1)$. By the similar arguments as for (S.39), we have that $\left|\frac{1}{n}\sum_{t=1}^{n}\sum_{t'>t} Cov\big(\varpi_t\varpi_{t'} \varsigma_{23nt}, \varsigma_{2nt'}\big)\right| = O\big(\frac{1}{\sqrt{n}l_n^{3/2}b^2}\big)$ and $\left|\frac{1}{n}\sum_{t=1}^{n}\sum_{t'>t} Cov(\varpi_t\varpi_{t'}, \varsigma_{24nt}\varsigma_{2nt'})\right| = O\big(\frac{1}{l_n^2b^2}\big)$. Hence,

$$\left|E\left(\frac{1}{n}\Xi_{14n}\right)\right| = O\left(\frac{1}{\sqrt{n}l_n^{3/2}b^2}\right) + O\left(\frac{1}{l_n^2b^2}\right). \tag{S.41}$$

Take $l_n = [b^{-(1+\delta_4)}]$ for some $\delta_4 > 0$. By (S.37)-(S.41) and Markov's inequality, we can obtain that

$$\frac{1}{n}\Xi_{1n} = O_p\left(\frac{1}{\sqrt{n}b^{\frac{5+\delta_4}{2}}} + \frac{1}{nb^{3+\delta_4}} + b^{\delta_4}\right).$$

Similarly, we can obtain the same results for $\frac{1}{n}\Xi_{2n}$ and $\frac{1}{n}\Xi_{3n}$, and together with (S.36), we can show that (i) holds. This completes all of the proofs. □

# REFERENCES

[1] Andrews, D.W.K. (1988) Laws of large numbers for dependent non-identically distributed random variables. *Econometr. Theor.* **4**, 458–467.

[2] Brockwell, P.J. and Davis, R.A. (1991) Time Series: Theory and Methods, second ed. Springer, New York.

[3] Davydov, Y.A. (1968) Convergence of distributions generated by stationary stochastic processes. *Theory Probab. Appl.* **13**, 691–696.

[4] Patilea, V. and Raïssi, H. (2014) Testing second-order dynamics for autoregressive processes in presence of time-varying variance. *J. Amer. Statist. Assoc.* **109**, 1099-1111.

[5] Pollard, D. (1991) Asymptotics for least absolute deviation regression estimators. *Econometr. Theor.* **7**, 186–199.

[6] Shao, Q.-M. and Yu, H. (1996) Weak convergence for weighted empirical processes of dependent sequences. *Ann. Probab.* **24**, 2098–2127.

[7] White, H. (2001) Asymptotic Theory for Econometricians: Revised Edition. Academic Press, New York.

[8] Xu, K.L. and Phillips, P.C.B. (2008) Adaptive estimation of autoregressive models with time-varying variances *J. Econometrics* **142**, 265–280.

University of Hong Kong
Department of Statistics and Actuarial Science
Pok Fu Lam Road
Hong Kong
E-mail: mazhuke@hku.hk
